# Supplementary material for: Chiral Pt(Me-BPCH): Synthesis and theoretical investigation of parity violation sensitivity
Source: arXiv:2509.26407 source file (2025-09-30)
Supplement: Supplementary file 1 [file Supplementary_Material.pdf]

## Supplementary Material

| Table of Contents                          | Pages |
|--------------------------------------------|-------|
| Experimental                               | 2     |
| Preparation and characterization details   | 2     |
| DSC thermal behavior for MeBPCH            | 3     |
| NMR for spectra for racemic MeBPCH         | 4-8   |
| NMR spectra for R,R'-MeBPCH                | 9-11  |
| NMR spectra for Pt(R,R'-MeBPCH)            | 12-14 |
| X-ray Crystallography                      | 15-22 |
| IR spectrum of PtMeBPCH                    | 23    |
| Proposed syntheses of PtMeBPCH analogs     | 24    |
| Computational                              | 25    |
| Optimized structure compared to experiment | 25    |
| Calculated PV vibrational frequency shifts | 27    |
| Vibrational modes overlaps                 | 33    |
| PV potential curve comparisons             | 36    |
| References                                 | 43    |

## Experimental

**Preparation of Me-BPCH.** The ligand was prepared by adapting a literature procedure [1]. In particular, to a solution of 6-Methylpyridine-2-carboxylic acid (750 mg, 5.46 mmol) in dichloromethane at 0 °C, oxalyl chloride (0.86 mL, 10 mmol, 1.8 eq.) was added dropwise followed by 2 drops of DMF. After stirring at room temperature for 5 hours, the volatiles were removed in vacuo. The residue was then resuspended in dichloromethane and cooled to 0 °C. To the mixture, (1R,2R)-1,2-diaminocyclohexane (312 mg, 2.73 mmol, 0.5 eq.) was added followed by triethylamine (2.788 mL, 20 mmol, 3.66 eq.). After 4 hours, the mixture was diluted with water and transferred to a separatory funnel. The organic phase was washed twice with water, once with saturated sodium bicarbonate, once again with water, and then with brine. The isolated organic layer was concentrated in vacuo, then purified through a silica plug in ethyl acetate. Yielding 906 mg of Me-BPCH as an orange oil (91% yield). Spectroscopic characterization identical to published results [1]. <sup>1</sup>H NMR (CDCl<sub>3</sub>): CH<sub>2</sub> 1.497(m, 2H); CH<sub>2</sub> 1.862(m, 1H); CH<sub>2</sub> 2.255(d, J=10.65 Hz, 1H); CH<sub>3</sub> 2.566(s, 3H); CH 4.071(m, 1H); CH 7.210(d, J=7.75 Hz 1H); CH 7.644(t, J=7.80 Hz, 1H); CH 7.906(d, J= 7.80 Hz, 1H); NH 8.349(s, 1H).

**Preparation of Pt(Me-BPCH).** Na<sub>2</sub>PtCl<sub>4</sub> (0.29 mmol, 109 mg) was dissolved in water and heated. R,R-MeBPCH (0.42 mmol, 148 mg) dissolved in a minimal amount of warm ethanol was added to the platinum solution. The mixture was left to reflux with stirring for 2.5 hours. The volume was then reduced by about half using rotary evaporation, and then left at -20 °C for 30 minutes to promote precipitation. The suspension was then filtered through a fritted funnel and washed with water. The collection flask was changed and the precipitate was washed through the frit with chloroform. The chloroform was dried over sodium sulfate and filtered. The solvent was then removed by rotary evaporation to yield 61mg of R,R-Pt(Me-BPCH) (39.4% yield). <sup>1</sup>H NMR (CDCl<sub>3</sub>): CH<sub>2</sub> 1.459(m, 2H); CH<sub>2</sub> 1.695(m, 1H); CH<sub>2</sub> 2.540(s, 3H); CH<sub>3</sub> 3.172(d, J =8.7 Hz, 1H); CH 3.880(m, 1H); CH 7.409(dd, J =7.95 Hz, J =1.5 Hz, 1H); CH 7.793(dd, J =7.65 Hz, J =1.85 Hz, 1H); CH 7.929(t, J =7.60 Hz, 1H).

## DSC thermal behavior for MeBPCH

Sample: MeBPCHrecrys

Size: 1.1000 mg

DSC

Run Date: 29-May-23 14:56  
Instrument: 2010 DSC V4.4E

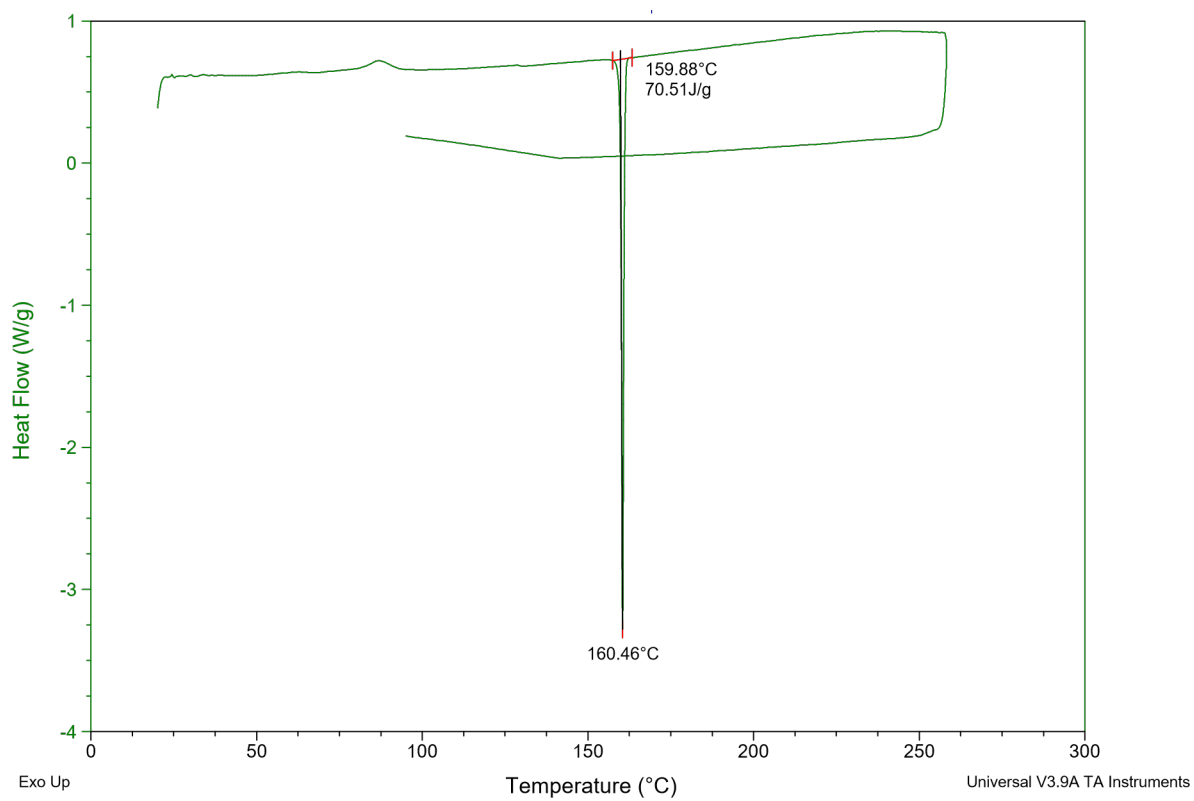

Figure S1: Racemic MeBPCH DSC

## NMR for spectra for racemic MeBPCH

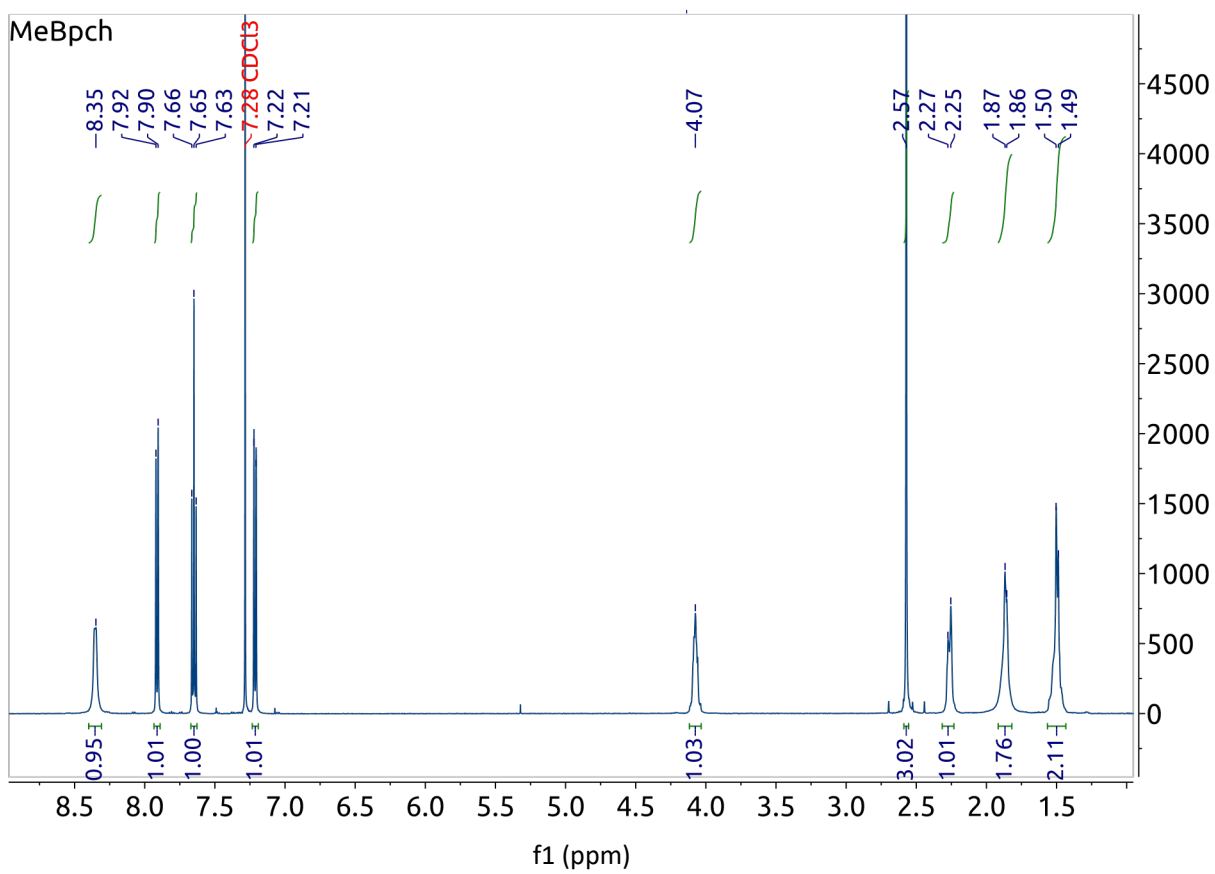

Figure S2: Racemic MeBPCH <sup>1</sup>H NMR

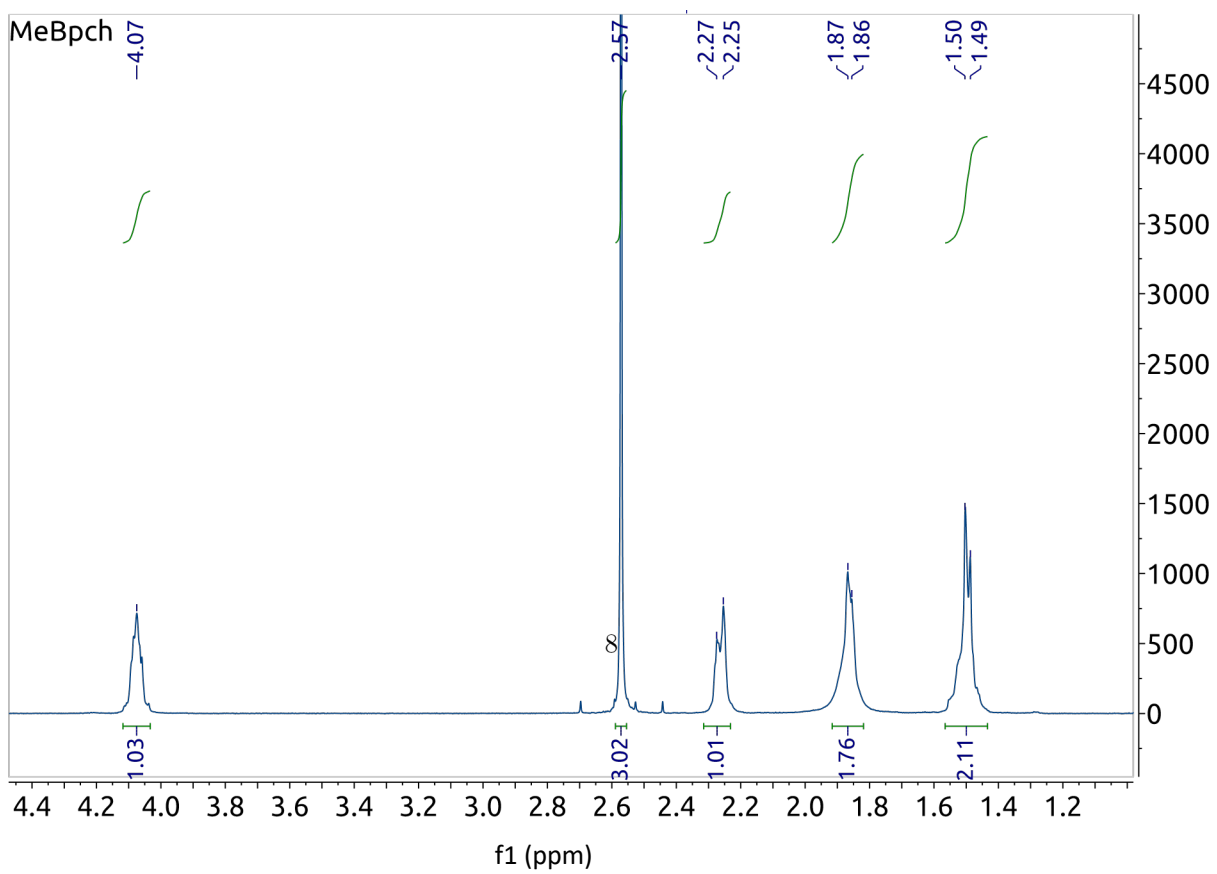

Figure S3: Racemic MeBPCH  $^1\text{H}$  NMR

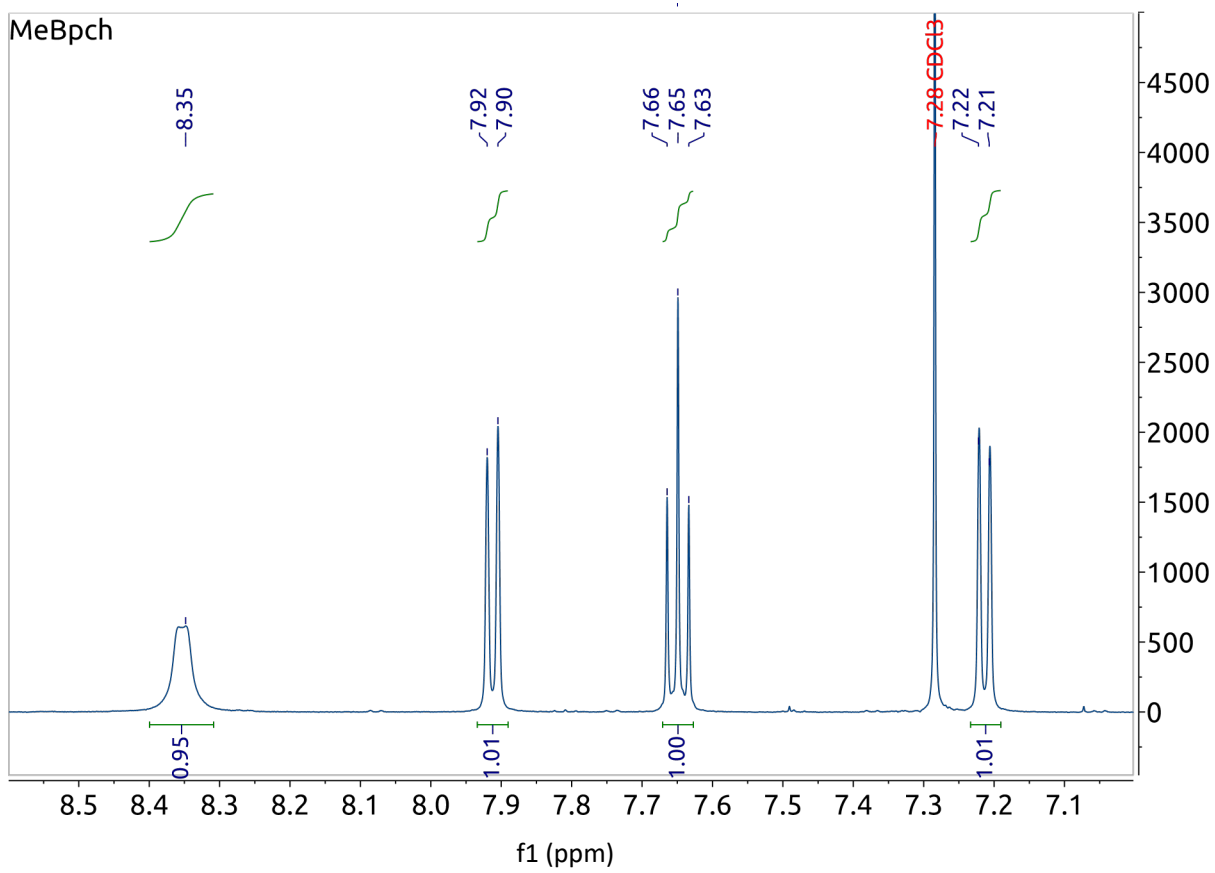

Figure S4: Racemic MeBPCH <sup>1</sup>H NMR

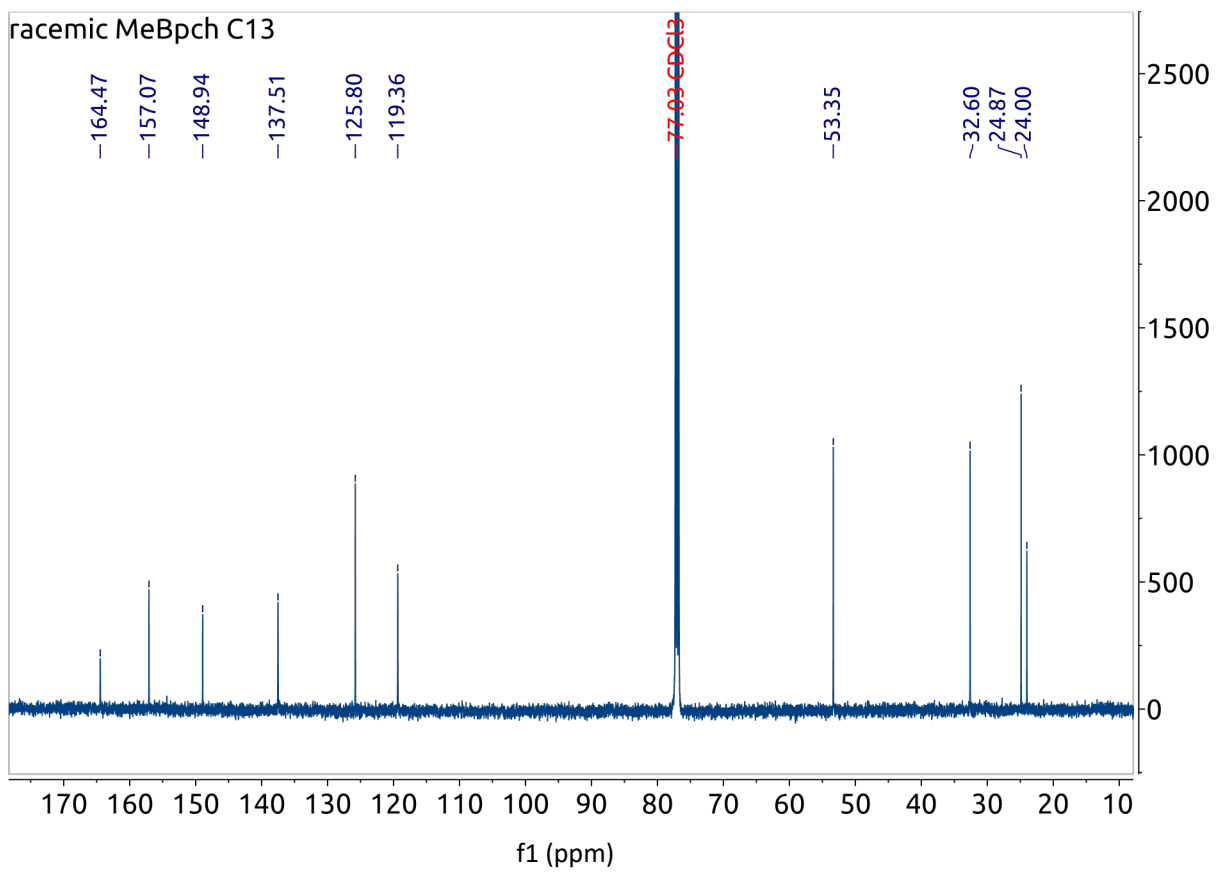

Figure S5: Racemic MeBPCH <sup>13</sup>C NMR

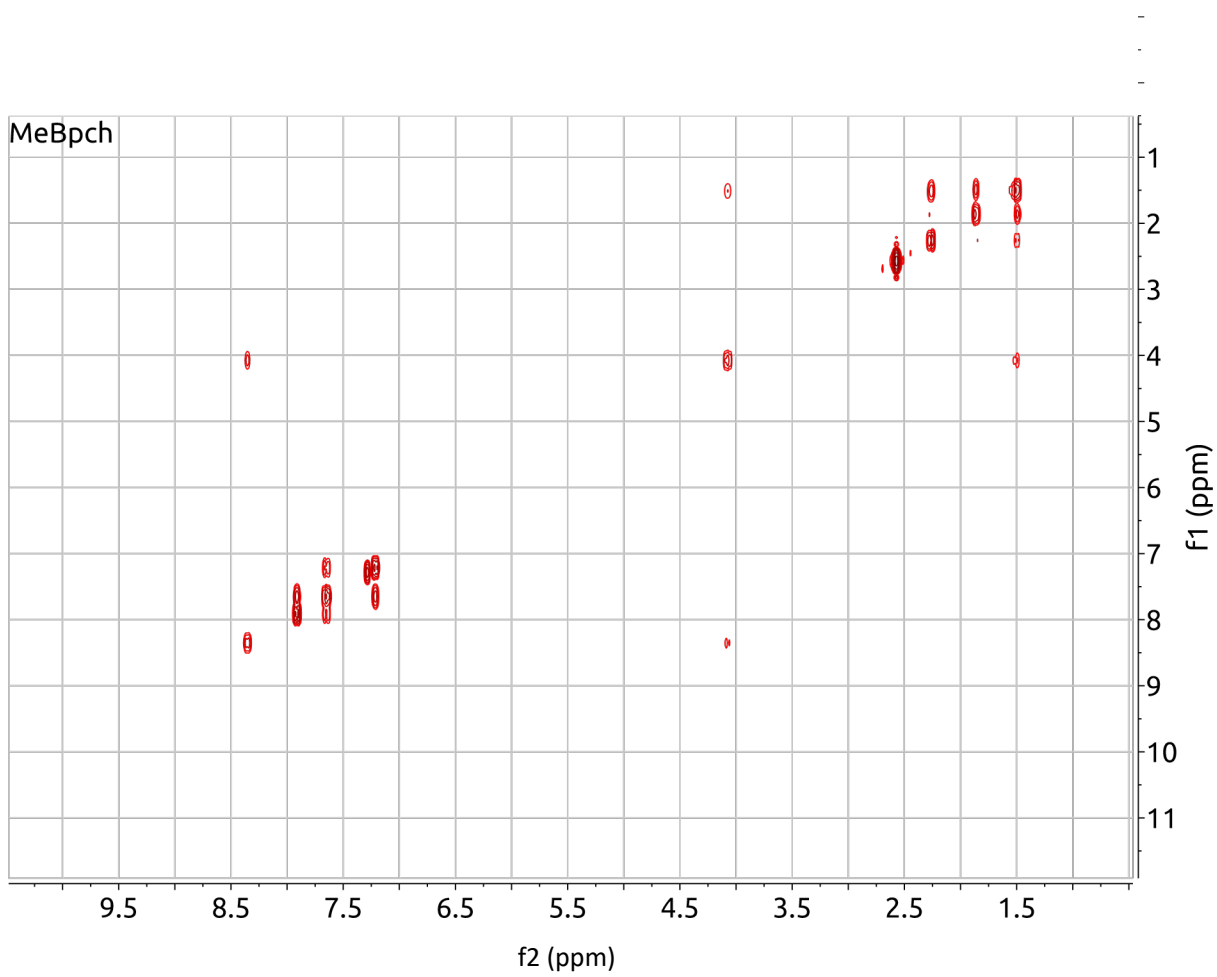

Figure S6: Racemic MeBPCH NMR COSY



## NMR spectra for R,R'-MeBPCH

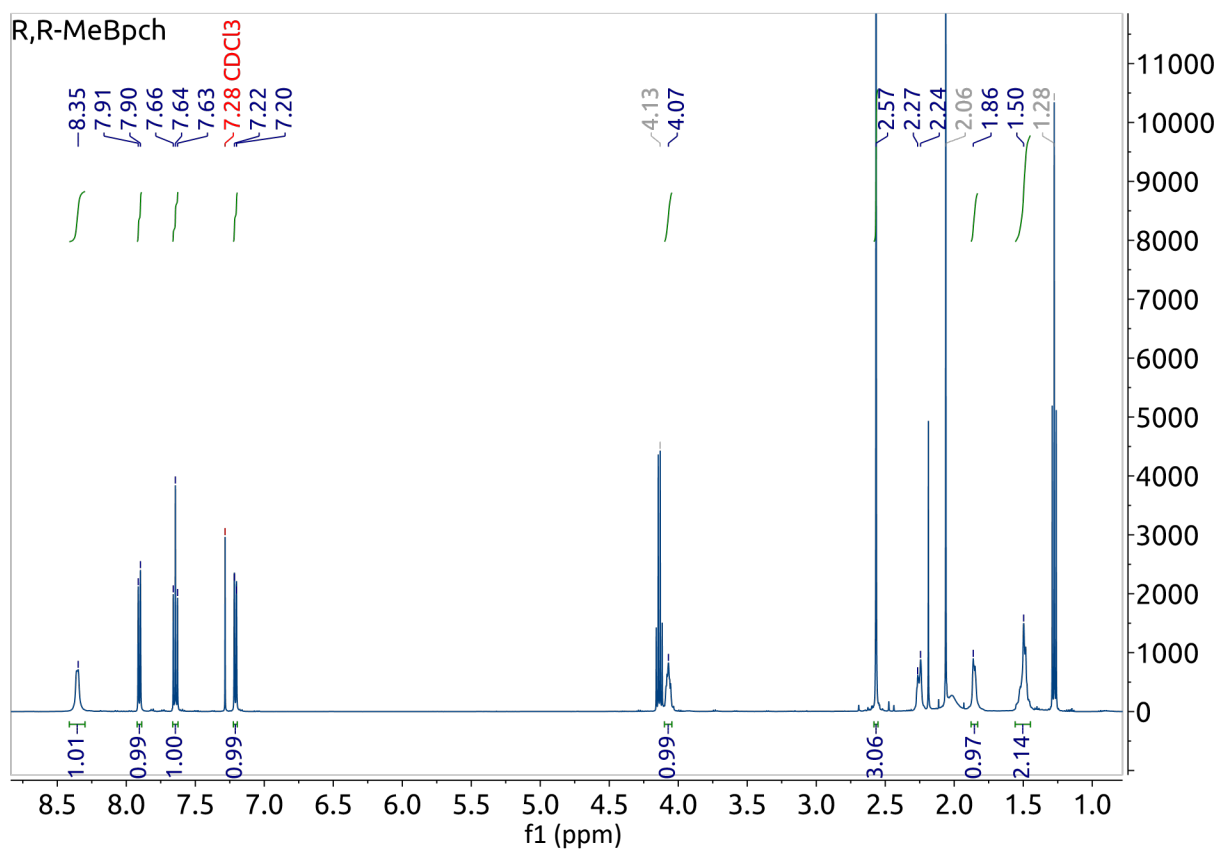

Figure S7: Racemic MeBPCH <sup>1</sup>H NMR

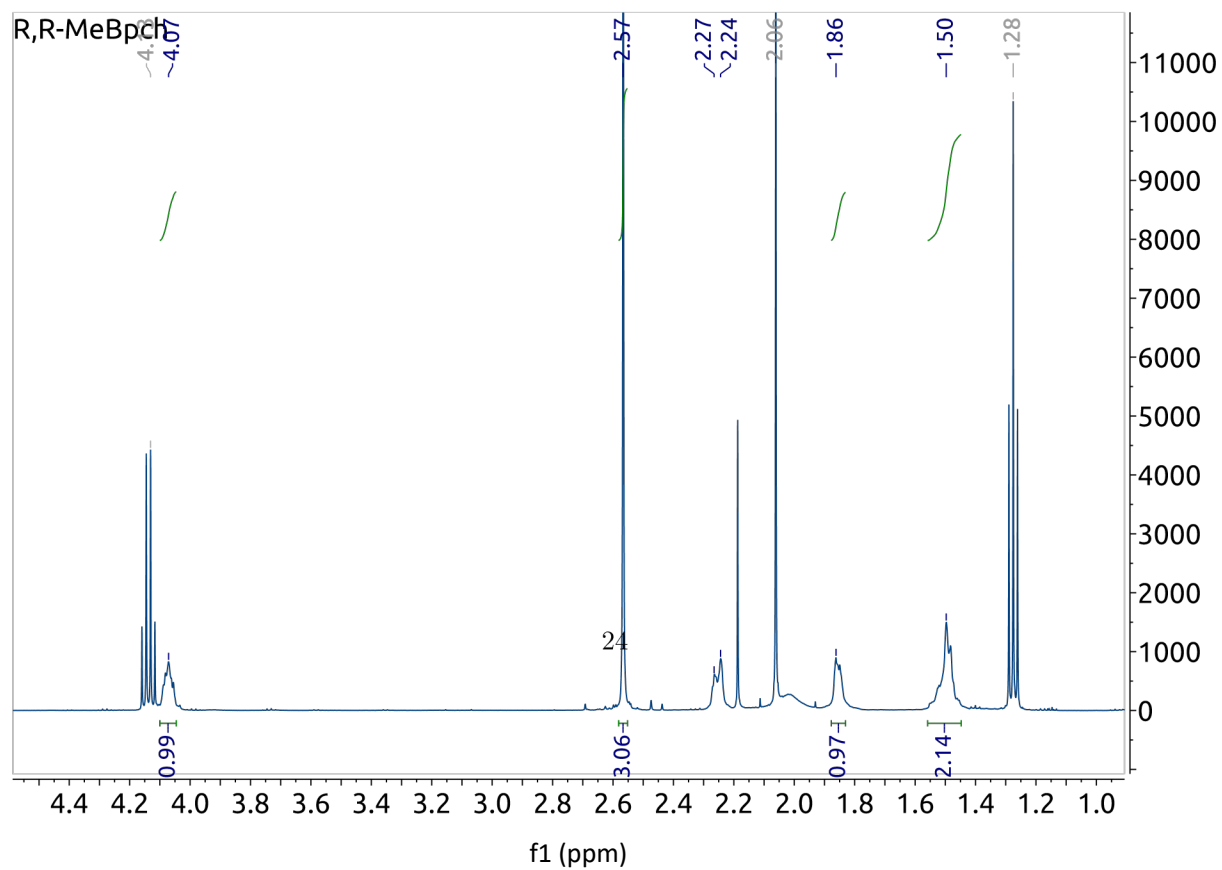

Figure S8: Racemic MeBPCH  $^1\text{H}$  NMR

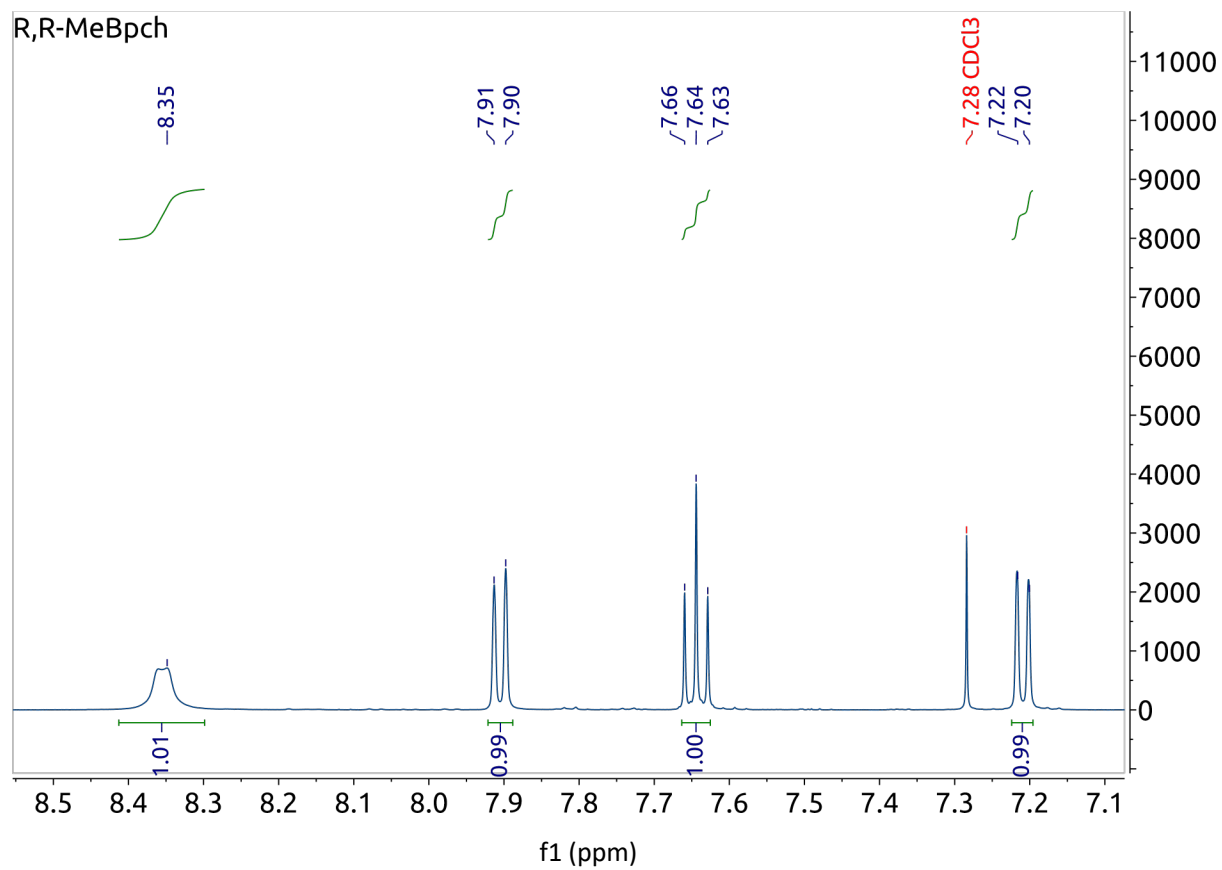

Figure S9: Enantiopure R,R-MeBPCH  $^1\text{H}$  NMR

## NMR spectra for Pt(R,R'-MeBPCH)

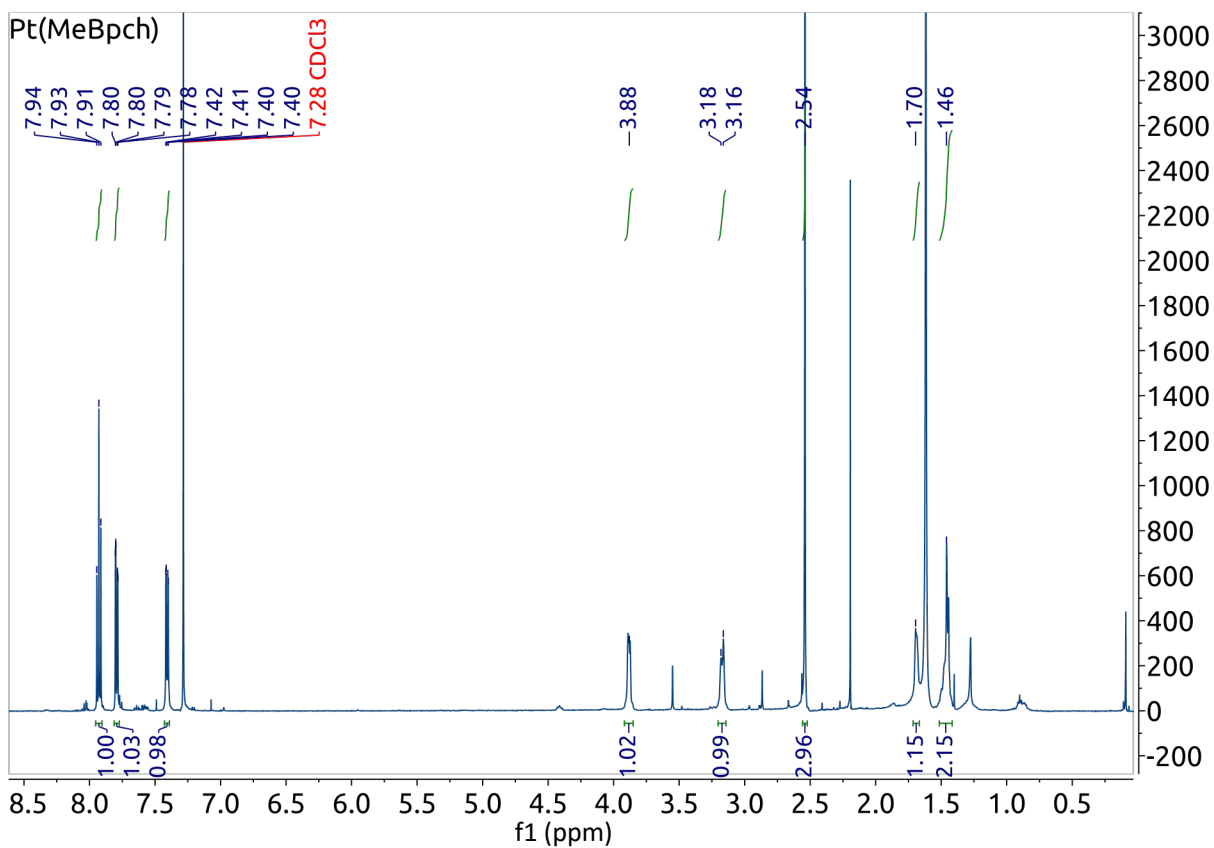

Figure S10: Enantiopure Pt(R,R-MeBPCH) <sup>1</sup>H NMR

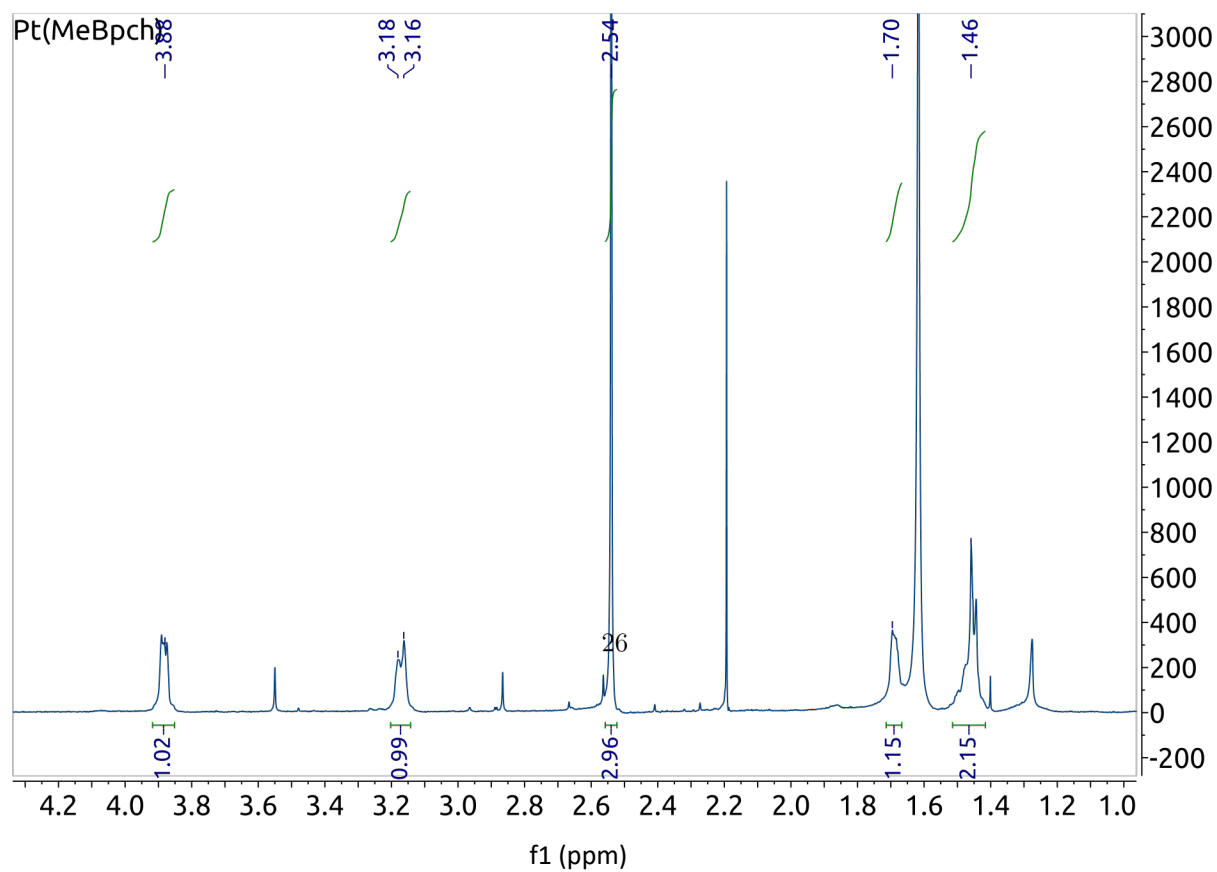

Figure S11: Enantiopure  $\text{Pt}(\text{R,R-MeBPCH})$   $^1\text{H}$  NMR

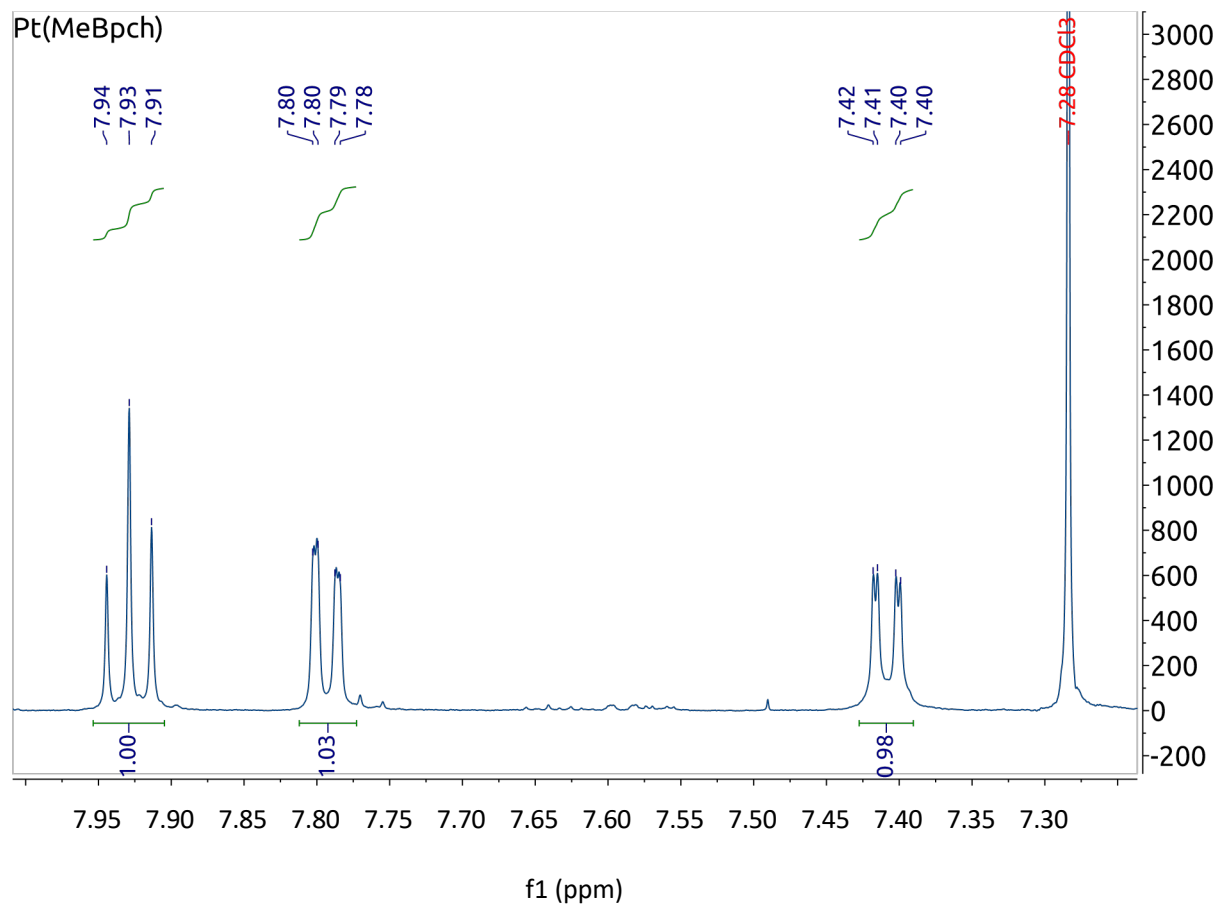

Figure S12: Enantiopure Pt(MeBPCH)  $^1\text{H}$  NMR

## X-ray Crystallography

The X-ray diffraction data were measured with graphite monochromated Mo  $K\alpha$  radiation ( $\lambda = 0.71073 \text{ \AA}$ ) with a Bruker D8 diffractometer on a crystal that was attached to a mitogen mount with viscous paratone N oil and cooled to 100 K. The structure was solved by direct methods and intrinsic phasing with the APEX 2 implementation platform provided by Bruker, on absorption-corrected data generated by SADABS. The resulting data set has a resolution of  $d = 0.84 \text{ \AA}$ . Refinement was achieved by a full-matrix least-squares procedure based on  $F^2$ . The noncentrosymmetric orthorhombic space group  $P2_12_12_1$  with the R,R setting for the cyclohexane substituents was confirmed with the calculated Flack parameter. Two independent molecules are present in the asymmetric unit with this constitution confirmed with the final refinement cycle having no correlation coefficients greater than 0.5. Crystallographic results have been deposited with the CCDB with CCDC number 2419012:

<https://www.ccdc.cam.ac.uk/structures/Search?Ccdcid=2419012>

# Crystal Structure Report for CS\_MeBPCH

A clear yellow needle-like specimen of  $C_{20}H_{22}N_4O_5Pt$ , approximate dimensions 0.300 mm x 0.300 mm x 0.800 mm, was used for the X-ray crystallographic analysis. The X-ray intensity data were measured.

Table S1: Data collection details for CS\_MeBPCH.

| Axis  | dx/mm  | 2 $\theta$ /° | $\omega$ /° | $\phi$ /° | $\chi$ /° | Width/° | Frames | Time/s | Wavelength/Å | Voltage/kV | Current/mA | Temperature/K |
|-------|--------|---------------|-------------|-----------|-----------|---------|--------|--------|--------------|------------|------------|---------------|
| Omega | 60.252 | -28.00        | -28.00      | 0.00      | 54.74     | 0.50    | 366    | 10.00  | 0.71073      | 50         | 30.0       | n/a           |
| Omega | 60.252 | -28.00        | -28.00      | 90.00     | 54.74     | 0.50    | 366    | 10.00  | 0.71073      | 50         | 30.0       | n/a           |
| Omega | 60.252 | -28.00        | -28.00      | 180.00    | 54.74     | 0.50    | 366    | 10.00  | 0.71073      | 50         | 30.0       | n/a           |
| Omega | 60.252 | -28.00        | -28.00      | 270.00    | 54.74     | 0.50    | 366    | 10.00  | 0.71073      | 50         | 30.0       | n/a           |

A total of 1464 frames were collected. The total exposure time was 4.07 hours. The frames were integrated with the Bruker SAINT software package using a narrow-frame algorithm. The integration of the data using an orthorhombic unit cell yielded a total of 41626 reflections to a maximum  $\theta$  angle of 25.06° (0.84 Å resolution), of which 7564 were independent (average redundancy 5.503, completeness = 99.6%,  $R_{int}$  = 4.47%,  $R_{sig}$  = 3.85%) and 6719 (88.83%) were greater than  $2\sigma(F^2)$ . The final cell constants of  $a$  = 8.2879(14) Å,  $b$  = 22.216(4) Å,  $c$  = 23.303(4) Å, volume = 4290.6(12) Å<sup>3</sup>, are based upon the refinement of the XYZ-centroids of 9949 reflections above 20  $\sigma(I)$  with 6.035° < 2 $\theta$  < 49.49°. Data were corrected for absorption effects using the multi-scan method (SADABS). The ratio of minimum to maximum apparent transmission was 0.566. The calculated minimum and maximum transmission coefficients (based on crystal size) are 0.0770 and 0.2430.

The final anisotropic full-matrix least-squares refinement on  $F^2$  with 541 variables converged at  $R1$  = 2.49%, for the observed data and  $wR2$  = 6.80% for all data. The goodness-of-fit was 1.088. The largest peak in the final difference electron density synthesis was 0.439 e<sup>-</sup>/Å<sup>3</sup> and the largest hole was -0.500 e<sup>-</sup>/Å<sup>3</sup> with an RMS deviation of 0.110 e<sup>-</sup>/Å<sup>3</sup>. On the basis of the final model, the calculated density was 1.838 g/cm<sup>3</sup> and  $F(000)$ , 2304 e<sup>-</sup>.



Table S2. Sample and crystal data for CS\_MeBPCH.

|                        |                                                                  |         |  |
|------------------------|------------------------------------------------------------------|---------|--|
| Identification code    | CS_MeBPCH                                                        |         |  |
| Chemical formula       | C <sub>20</sub> H <sub>22</sub> N <sub>4</sub> O <sub>5</sub> Pt |         |  |
| Formula weight         | 593.50 g/mol                                                     |         |  |
| Temperature            | 295(2) K                                                         |         |  |
| Wavelength             | 0.71073 Å                                                        |         |  |
| Crystal size           | 0.300 x 0.300 x 0.800 mm                                         |         |  |
| Crystal habit          | clear yellow needle                                              |         |  |
| Crystal system         | orthorhombic                                                     |         |  |
| Space group            | P 21 21 21                                                       |         |  |
| Unit cell dimensions   | a = 8.2879(14) Å                                                 | α = 90° |  |
|                        | b = 22.216(4) Å                                                  | β = 90° |  |
|                        | c = 23.303(4) Å                                                  | γ = 90° |  |
| Volume                 | 4290.6(12) Å <sup>3</sup>                                        |         |  |
| Z                      | 8                                                                |         |  |
| Density (calculated)   | 1.838 g/cm <sup>3</sup>                                          |         |  |
| Absorption coefficient | 6.579 mm <sup>-1</sup>                                           |         |  |
| F(000)                 | 2304                                                             |         |  |

Table 3. Data collection and structure refinement for CS\_MeBPCH.

|                                     |                                             |                           |
|-------------------------------------|---------------------------------------------|---------------------------|
| Theta range for data collection     | 1.27 to 25.06°                              |                           |
| Index ranges                        | -9<=h<=9, -26<=k<=26, -27<=l<=27            |                           |
| Reflections collected               | 41626                                       |                           |
| Independent reflections             | 7564 [R(int) = 0.0447]                      |                           |
| Coverage of independent reflections | 99.6%                                       |                           |
| Absorption correction               | multi-scan                                  |                           |
| Max. and min. transmission          | 0.2430 and 0.0770                           |                           |
| Refinement method                   | Full-matrix least-squares on F <sup>2</sup> |                           |
| Refinement program                  | SHELXL-2014/7 (Sheldrick, 2014)             |                           |
| Function minimized                  | $\Sigma w(F_o^2 - F_c^2)^2$                 |                           |
| Data / restraints / parameters      | 7564 / 0 / 541                              |                           |
| Goodness-of-fit on F <sup>2</sup>   | 1.088                                       |                           |
| $\Delta/\sigma_{\max}$              | 0.001                                       |                           |
| Final R indices                     | 6719 data; I>2σ(I)                          | R1 = 0.0249, wR2 = 0.0607 |
|                                     | all data                                    | R1 = 0.0315, wR2 = 0.0680 |
| Weighting scheme                    | $w=1/[\sigma^2(F_o^2)+(0.0274P)^2+2.9168P]$ |                           |
|                                     | where $P=(F_o^2+2F_c^2)/3$                  |                           |
| Absolute structure parameter        | 0.0(0)                                      |                           |
| Largest diff. peak and hole         | 0.439 and -0.500 eÅ <sup>-3</sup>           |                           |
| R.M.S. deviation from mean          | 0.110 eÅ <sup>-3</sup>                      |                           |

Table S4. Atomic coordinates and equivalent isotropic atomic displacement parameters (Å<sup>2</sup>) for CS\_MeBPCH.

U(eq) is defined as one third of the trace of the orthogonalized U<sub>ij</sub> tensor.

|      | x/a        | y/b        | z/c        | U(eq)       |
|------|------------|------------|------------|-------------|
| Pt1A | 0.65451(3) | 0.74427(2) | 0.30879(2) | 0.02691(10) |
| Pt1  | 0.12216(4) | 0.74409(2) | 0.19662(2) | 0.02717(10) |
| O1   | 0.0438(9)  | 0.9199(3)  | 0.1727(3)  | 0.0411(18)  |
| N3A  | 0.6916(9)  | 0.6522(3)  | 0.3135(3)  | 0.0310(19)  |
| N3   | 0.0901(10) | 0.6522(3)  | 0.2024(4)  | 0.037(2)    |
| O1A  | 0.6892(9)  | 0.9253(3)  | 0.3125(3)  | 0.0539(19)  |
| C25A | 0.5939(12) | 0.7646(5)  | 0.4397(4)  | 0.038(2)    |
| C24  | 0.2114(13) | 0.7804(5)  | 0.0147(4)  | 0.045(3)    |
| O2A  | 0.5209(9)  | 0.6474(3)  | 0.1730(3)  | 0.0447(19)  |
| C2   | 0.0937(12) | 0.8668(4)  | 0.1698(4)  | 0.033(2)    |
| C31A | 0.6315(11) | 0.6249(5)  | 0.2649(4)  | 0.033(2)    |
| N4   | 0.1479(9)  | 0.7754(4)  | 0.1135(3)  | 0.033(2)    |
| C22  | 0.1248(14) | 0.8676(5)  | 0.0619(4)  | 0.046(3)    |
| N2   | 0.1401(9)  | 0.7342(3)  | 0.2797(3)  | 0.0327(19)  |
| C21A | 0.6651(12) | 0.8466(4)  | 0.3813(4)  | 0.033(2)    |
| C3A  | 0.5854(12) | 0.6668(4)  | 0.2157(5)  | 0.032(2)    |
| C2A  | 0.6656(12) | 0.8718(4)  | 0.3210(5)  | 0.037(3)    |
| N1A  | 0.6350(9)  | 0.7236(3)  | 0.2269(3)  | 0.0292(19)  |
| O4S  | 0.4312(11) | 0.5328(4)  | 0.1220(3)  | 0.068(2)    |
| C31  | 0.1509(12) | 0.6333(5)  | 0.2542(5)  | 0.036(3)    |
| C35A | 0.7646(12) | 0.6177(4)  | 0.3538(4)  | 0.037(2)    |
| N1   | 0.1378(10) | 0.8310(3)  | 0.2127(3)  | 0.030(2)    |
| N4A  | 0.6352(9)  | 0.7865(3)  | 0.3875(3)  | 0.0303(19)  |

|      | x/a        | y/b       | z/c       | U(eq)    |
|------|------------|-----------|-----------|----------|
| C26  | 0.2688(13) | 0.6859(4) | 0.0697(4) | 0.044(3) |
| N2A  | 0.6320(10) | 0.8289(4) | 0.2830(4) | 0.032(2) |
| C15A | 0.5770(12) | 0.8885(4) | 0.1925(4) | 0.040(2) |
| C33A | 0.6827(13) | 0.5281(5) | 0.3040(5) | 0.052(3) |
| C3   | 0.1956(12) | 0.6805(4) | 0.2971(4) | 0.034(2) |
| C24A | 0.6089(14) | 0.8019(5) | 0.4877(4) | 0.047(3) |
| O1S  | 0.3521(10) | 0.5642(3) | 0.3997(4) | 0.069(2) |
| C13  | 0.1568(14) | 0.9091(4) | 0.3597(4) | 0.044(3) |
| C12  | 0.1954(13) | 0.9017(4) | 0.2959(4) | 0.037(2) |
| C23A | 0.6579(14) | 0.8595(5) | 0.4825(5) | 0.052(3) |
| C22A | 0.6805(13) | 0.8839(5) | 0.4282(5) | 0.046(3) |
| C11A | 0.5864(11) | 0.7765(4) | 0.1916(4) | 0.029(2) |
| O2   | 0.2614(9)  | 0.6677(3) | 0.3425(3) | 0.051(2) |
| O3S  | 0.0902(9)  | 0.4941(3) | 0.4210(3) | 0.061(2) |
| C21  | 0.1169(12) | 0.8364(5) | 0.1126(4) | 0.036(2) |
| C23  | 0.1675(15) | 0.8393(5) | 0.0122(4) | 0.054(3) |
| C11  | 0.1168(12) | 0.8441(4) | 0.2739(4) | 0.029(2) |
| O5S  | 0.2094(12) | 0.5416(4) | 0.0229(4) | 0.088(3) |
| C16  | 0.1867(12) | 0.7918(4) | 0.3081(4) | 0.033(2) |
| C13A | 0.5703(14) | 0.8305(5) | 0.0987(4) | 0.043(3) |
| O6S  | 0.6283(11) | 0.4969(5) | 0.0206(4) | 0.098(4) |
| C32  | 0.1614(13) | 0.5731(4) | 0.2677(5) | 0.046(3) |
| C35  | 0.0186(12) | 0.6127(4) | 0.1656(5) | 0.037(2) |
| C14A | 0.6180(14) | 0.8888(5) | 0.1282(4) | 0.049(3) |
| C14  | 0.2050(15) | 0.8559(4) | 0.3957(4) | 0.046(3) |
| C34A | 0.7573(13) | 0.5557(4) | 0.3494(5) | 0.048(3) |
| C33  | 0.1015(14) | 0.5302(5) | 0.2288(5) | 0.056(3) |
| C12A | 0.6352(13) | 0.7748(4) | 0.1297(4) | 0.041(3) |
| C34  | 0.0254(14) | 0.5517(5) | 0.1793(5) | 0.056(3) |
| C36A | 0.8627(12) | 0.6469(4) | 0.3995(4) | 0.045(3) |
| C32A | 0.6221(13) | 0.5629(5) | 0.2604(5) | 0.044(3) |
| O2S  | 0.5486(14) | 0.5366(6) | 0.4898(5) | 0.117(4) |
| C16A | 0.6503(12) | 0.8333(4) | 0.2207(4) | 0.031(2) |
| C26A | 0.5255(14) | 0.7027(5) | 0.4443(4) | 0.049(3) |
| C36  | 0.9207(13) | 0.6349(5) | 0.1159(4) | 0.051(3) |
| C15  | 0.1376(14) | 0.7966(4) | 0.3709(4) | 0.042(3) |
| C25  | 0.2038(11) | 0.7485(5) | 0.0660(4) | 0.037(2) |

**Table S5. Bond lengths (Å) for CS\_MeBPCH.**

|           |           |           |           |
|-----------|-----------|-----------|-----------|
| Pt1A-N1A  | 1.969(8)  | Pt1A-N2A  | 1.982(8)  |
| Pt1A-N4A  | 2.066(7)  | Pt1A-N3A  | 2.070(7)  |
| Pt1-N2    | 1.954(7)  | Pt1-N1    | 1.971(8)  |
| Pt1-N3    | 2.064(7)  | Pt1-N4    | 2.069(7)  |
| O1-C2     | 1.251(11) | N3A-C35A  | 1.355(11) |
| N3A-C31A  | 1.377(12) | N3-C35    | 1.361(12) |
| N3-C31    | 1.374(13) | O1A-C2A   | 1.221(11) |
| C25A-N4A  | 1.356(11) | C25A-C24A | 1.397(13) |
| C25A-C26A | 1.491(15) | C24-C23   | 1.360(14) |
| C24-C25   | 1.390(12) | C24-H24A  | 0.93      |
| O2A-C3A   | 1.209(12) | C2-N1     | 1.327(12) |
| C2-C21    | 1.507(14) | C31A-C32A | 1.384(14) |
| C31A-C3A  | 1.527(14) | N4-C25    | 1.339(11) |
| N4-C21    | 1.380(12) | C22-C23   | 1.364(14) |
| C22-C21   | 1.370(13) | C22-H22A  | 0.93      |
| N2-C3     | 1.343(11) | N2-C16    | 1.491(11) |
| C21A-N4A  | 1.365(12) | C21A-C22A | 1.376(13) |
| C21A-C2A  | 1.513(14) | C3A-N1A   | 1.351(11) |
| C2A-N2A   | 1.330(13) | N1A-C11A  | 1.491(10) |
| C31-C32   | 1.378(14) | C31-C3    | 1.495(14) |
| C35A-C34A | 1.384(13) | C35A-C36A | 1.487(13) |
| N1-C11    | 1.467(13) | C26-C25   | 1.494(14) |
| C26-H26A  | 0.96      | C26-H26B  | 0.96      |
| C26-H26C  | 0.96      | N2A-C16A  | 1.464(14) |
| C15A-C16A | 1.517(13) | C15A-C14A | 1.536(13) |
| C15A-H15A | 0.97      | C15A-H15B | 0.97      |
| C33A-C32A | 1.371(14) | C33A-C34A | 1.371(14) |
| C33A-H33A | 0.93      | C3-O2     | 1.224(11) |
| C24A-C23A | 1.347(15) | C24A-H24B | 0.93      |
| C13-C14   | 1.504(13) | C13-C12   | 1.528(13) |
| C13-H13A  | 0.97      | C13-H13B  | 0.97      |
| C12-C11   | 1.525(12) | C12-H12A  | 0.97      |
| C12-H12B  | 0.97      | C23A-C22A | 1.390(15) |
| C23A-H23A | 0.93      | C22A-H22B | 0.93      |
| C11A-C12A | 1.499(12) | C11A-C16A | 1.527(12) |
| C11A-H11A | 0.98      | C23-H23B  | 0.93      |
| C11-C16   | 1.522(12) | C11-H11B  | 0.98      |

|           |           |           |           |
|-----------|-----------|-----------|-----------|
| C16-C15   | 1.522(12) | C16-H16A  | 0.98      |
| C13A-C14A | 1.518(14) | C13A-C12A | 1.531(12) |
| C13A-H13C | 0.97      | C13A-H13D | 0.97      |
| C32-C33   | 1.407(15) | C32-H32A  | 0.93      |
| C35-C34   | 1.393(13) | C35-C36   | 1.499(14) |
| C14A-H14A | 0.97      | C14A-H14B | 0.97      |
| C14-C15   | 1.543(13) | C14-H14C  | 0.97      |
| C14-H14D  | 0.97      | C34A-H34A | 0.93      |
| C33-C34   | 1.399(15) | C33-H33B  | 0.93      |
| C12A-H12C | 0.97      | C12A-H12D | 0.97      |
| C34-H34B  | 0.93      | C36A-H36A | 0.96      |
| C36A-H36B | 0.96      | C36A-H36C | 0.96      |
| C32A-H32B | 0.93      | C16A-H16B | 0.98      |
| C26A-H26D | 0.96      | C26A-H26E | 0.96      |
| C26A-H26F | 0.96      | C36-H36D  | 0.96      |
| C36-H36E  | 0.96      | C36-H36F  | 0.96      |
| C15-H15C  | 0.97      | C15-H15D  | 0.97      |

**Table S6. Bond angles (°) for CS\_MeBPCH.**

|                |           |                |           |
|----------------|-----------|----------------|-----------|
| N1A-Pt1A-N2A   | 85.4(3)   | N1A-Pt1A-N4A   | 163.6(3)  |
| N2A-Pt1A-N4A   | 80.2(3)   | N1A-Pt1A-N3A   | 80.4(3)   |
| N2A-Pt1A-N3A   | 165.1(3)  | N4A-Pt1A-N3A   | 114.4(3)  |
| N2-Pt1-N1      | 85.2(3)   | N2-Pt1-N3      | 80.5(3)   |
| N1-Pt1-N3      | 164.9(3)  | N2-Pt1-N4      | 163.2(3)  |
| N1-Pt1-N4      | 80.9(3)   | N3-Pt1-N4      | 114.0(3)  |
| C35A-N3A-C31A  | 118.8(8)  | C35A-N3A-Pt1A  | 131.4(6)  |
| C31A-N3A-Pt1A  | 109.8(6)  | C35-N3-C31     | 121.1(9)  |
| C35-N3-Pt1     | 130.7(7)  | C31-N3-Pt1     | 108.1(7)  |
| N4A-C25A-C24A  | 118.8(10) | N4A-C25A-C26A  | 119.4(9)  |
| C24A-C25A-C26A | 121.7(9)  | C23-C24-C25    | 121.0(10) |
| C23-C24-H24A   | 119.5     | C25-C24-H24A   | 119.5     |
| O1-C2-N1       | 127.9(9)  | O1-C2-C21      | 120.8(9)  |
| N1-C2-C21      | 111.2(8)  | N3A-C31A-C32A  | 121.4(9)  |
| N3A-C31A-C3A   | 116.1(9)  | C32A-C31A-C3A  | 122.4(9)  |
| C25-N4-C21     | 119.3(8)  | C25-N4-Pt1     | 131.2(7)  |
| C21-N4-Pt1     | 109.0(6)  | C23-C22-C21    | 120.8(11) |
| C23-C22-H22A   | 119.6     | C21-C22-H22A   | 119.6     |
| C3-N2-C16      | 122.7(7)  | C3-N2-Pt1      | 115.2(7)  |
| C16-N2-Pt1     | 111.3(5)  | N4A-C21A-C22A  | 121.5(9)  |
| N4A-C21A-C2A   | 117.3(8)  | C22A-C21A-C2A  | 120.9(9)  |
| O2A-C3A-N1A    | 128.8(9)  | O2A-C3A-C31A   | 120.8(9)  |
| N1A-C3A-C31A   | 110.3(9)  | O1A-C2A-N2A    | 128.6(10) |
| O1A-C2A-C21A   | 120.7(9)  | N2A-C2A-C21A   | 110.6(8)  |
| C3A-N1A-C11A   | 123.1(8)  | C3A-N1A-Pt1A   | 115.5(6)  |
| C11A-N1A-Pt1A  | 111.9(5)  | N3-C31-C32     | 121.3(10) |
| N3-C31-C3      | 117.8(9)  | C32-C31-C3     | 120.8(10) |
| N3A-C35A-C34A  | 119.5(9)  | N3A-C35A-C36A  | 119.6(8)  |
| C34A-C35A-C36A | 120.7(9)  | C2-N1-C11      | 125.5(8)  |
| C2-N1-Pt1      | 115.2(7)  | C11-N1-Pt1     | 111.8(5)  |
| C25A-N4A-C21A  | 119.4(8)  | C25A-N4A-Pt1A  | 130.8(7)  |
| C21A-N4A-Pt1A  | 109.7(6)  | C25-C26-H26A   | 109.5     |
| C25-C26-H26B   | 109.5     | H26A-C26-H26B  | 109.5     |
| C25-C26-H26C   | 109.5     | H26A-C26-H26C  | 109.5     |
| H26B-C26-H26C  | 109.5     | C2A-N2A-C16A   | 126.2(8)  |
| C2A-N2A-Pt1A   | 117.3(7)  | C16A-N2A-Pt1A  | 110.8(5)  |
| C16A-C15A-C14A | 109.7(8)  | C16A-C15A-H15A | 109.7     |
| C14A-C15A-H15A | 109.7     | C16A-C15A-H15B | 109.7     |
| C14A-C15A-H15B | 109.7     | H15A-C15A-H15B | 108.2     |
| C32A-C33A-C34A | 119.0(10) | C32A-C33A-H33A | 120.5     |
| C34A-C33A-H33A | 120.5     | O2-C3-N2       | 128.4(9)  |
| O2-C3-C31      | 121.7(9)  | N2-C3-C31      | 109.6(9)  |
| C23A-C24A-C25A | 121.3(10) | C23A-C24A-H24B | 119.4     |
| C25A-C24A-H24B | 119.4     | C14-C13-C12    | 113.7(8)  |
| C14-C13-H13A   | 108.8     | C12-C13-H13A   | 108.8     |
| C14-C13-H13B   | 108.8     | C12-C13-H13B   | 108.8     |
| H13A-C13-H13B  | 107.7     | C11-C12-C13    | 109.1(8)  |
| C11-C12-H12A   | 109.9     | C13-C12-H12A   | 109.9     |
| C11-C12-H12B   | 109.9     | C13-C12-H12B   | 109.9     |
| H12A-C12-H12B  | 108.3     | C24A-C23A-C22A | 119.5(10) |
| C24A-C23A-H23A | 120.2     | C22A-C23A-H23A | 120.2     |
| C21A-C22A-C23A | 118.4(10) | C21A-C22A-H22B | 120.8     |
| C23A-C22A-H22B | 120.8     | N1A-C11A-C12A  | 116.0(7)  |
| N1A-C11A-C16A  | 108.3(7)  | C12A-C11A-C16A | 110.8(7)  |
| N1A-C11A-H11A  | 107.1     | C12A-C11A-H11A | 107.1     |
| C16A-C11A-H11A | 107.1     | C22-C21-N4     | 120.0(10) |
| C22-C21-C2     | 122.9(10) | N4-C21-C2      | 116.8(8)  |
| C24-C23-C22    | 118.4(10) | C24-C23-H23B   | 120.8     |

|                |           |                |           |
|----------------|-----------|----------------|-----------|
| C22-C23-H23B   | 120.8     | N1-C11-C16     | 108.2(7)  |
| N1-C11-C12     | 116.3(8)  | C16-C11-C12    | 107.6(8)  |
| N1-C11-H11B    | 108.2     | C16-C11-H11B   | 108.2     |
| C12-C11-H11B   | 108.2     | N2-C16-C15     | 114.6(7)  |
| N2-C16-C11     | 108.9(7)  | C15-C16-C11    | 110.3(8)  |
| N2-C16-H16A    | 107.6     | C15-C16-H16A   | 107.6     |
| C11-C16-H16A   | 107.6     | C14A-C13A-C12A | 112.6(8)  |
| C14A-C13A-H13C | 109.1     | C12A-C13A-H13C | 109.1     |
| C14A-C13A-H13D | 109.1     | C12A-C13A-H13D | 109.1     |
| H13C-C13A-H13D | 107.8     | C31-C32-C33    | 119.3(11) |
| C31-C32-H32A   | 120.4     | C33-C32-H32A   | 120.4     |
| N3-C35-C34     | 117.7(10) | N3-C35-C36     | 120.7(8)  |
| C34-C35-C36    | 121.3(9)  | C13A-C14A-C15A | 112.3(8)  |
| C13A-C14A-H14A | 109.1     | C15A-C14A-H14A | 109.1     |
| C13A-C14A-H14B | 109.1     | C15A-C14A-H14B | 109.1     |
| H14A-C14A-H14B | 107.9     | C13-C14-C15    | 111.5(8)  |
| C13-C14-H14C   | 109.3     | C15-C14-H14C   | 109.3     |
| C13-C14-H14D   | 109.3     | C15-C14-H14D   | 109.3     |
| H14C-C14-H14D  | 108.0     | C33A-C34A-C35A | 121.4(9)  |
| C33A-C34A-H34A | 119.3     | C35A-C34A-H34A | 119.3     |
| C34-C33-C32    | 117.3(9)  | C34-C33-H33B   | 121.4     |
| C32-C33-H33B   | 121.4     | C11A-C12A-C13A | 109.8(8)  |
| C11A-C12A-H12C | 109.7     | C13A-C12A-H12C | 109.7     |
| C11A-C12A-H12D | 109.7     | C13A-C12A-H12D | 109.7     |
| H12C-C12A-H12D | 108.2     | C35-C34-C33    | 122.6(10) |
| C35-C34-H34B   | 118.7     | C33-C34-H34B   | 118.7     |
| C35A-C36A-H36A | 109.5     | C35A-C36A-H36B | 109.5     |
| H36A-C36A-H36B | 109.5     | C35A-C36A-H36C | 109.5     |
| H36A-C36A-H36C | 109.5     | H36B-C36A-H36C | 109.5     |
| C33A-C32A-C31A | 119.0(10) | C33A-C32A-H32B | 120.5     |
| C31A-C32A-H32B | 120.5     | N2A-C16A-C15A  | 116.3(8)  |
| N2A-C16A-C11A  | 110.4(7)  | C15A-C16A-C11A | 109.7(8)  |
| N2A-C16A-H16B  | 106.7     | C15A-C16A-H16B | 106.7     |
| C11A-C16A-H16B | 106.7     | C25A-C26A-H26D | 109.5     |
| C25A-C26A-H26E | 109.5     | H26D-C26A-H26E | 109.5     |
| C25A-C26A-H26F | 109.5     | H26D-C26A-H26F | 109.5     |
| H26E-C26A-H26F | 109.5     | C35-C36-H36D   | 109.5     |
| C35-C36-H36E   | 109.5     | H36D-C36-H36E  | 109.5     |
| C35-C36-H36F   | 109.5     | H36D-C36-H36F  | 109.5     |
| H36E-C36-H36F  | 109.5     | C16-C15-C14    | 108.8(8)  |
| C16-C15-H15C   | 109.9     | C14-C15-H15C   | 109.9     |
| C16-C15-H15D   | 109.9     | C14-C15-H15D   | 109.9     |
| H15C-C15-H15D  | 108.3     | N4-C25-C24     | 119.9(10) |
| N4-C25-C26     | 119.5(8)  | C24-C25-C26    | 120.4(9)  |

**Table S7. Anisotropic atomic displacement parameters (Å<sup>2</sup>) for CS\_MeBPCH.**

The anisotropic atomic displacement factor exponent takes the form: -2π<sup>2</sup>[ h<sup>2</sup> a<sup>\*2</sup> U<sub>11</sub> + ... + 2 h k a<sup>\*</sup> b<sup>\*</sup> U<sub>12</sub> ]

|      | U <sub>11</sub> | U <sub>22</sub> | U <sub>33</sub> | U <sub>23</sub> | U <sub>13</sub> | U <sub>12</sub> |
|------|-----------------|-----------------|-----------------|-----------------|-----------------|-----------------|
| Pt1A | 0.03001(17)     | 0.0255(2)       | 0.02526(18)     | -0.00027(19)    | -0.00051(13)    | -0.00112(15)    |
| Pt1  | 0.03037(17)     | 0.02295(19)     | 0.02820(18)     | 0.00111(19)     | -0.00044(14)    | 0.00067(15)     |
| O1   | 0.058(5)        | 0.027(4)        | 0.039(4)        | 0.003(3)        | -0.008(4)       | 0.004(3)        |
| N3A  | 0.025(4)        | 0.032(4)        | 0.036(5)        | 0.000(4)        | -0.005(4)       | -0.001(3)       |
| N3   | 0.037(5)        | 0.023(4)        | 0.051(6)        | -0.002(4)       | 0.002(5)        | 0.002(4)        |
| O1A  | 0.084(5)        | 0.033(4)        | 0.044(4)        | 0.001(4)        | 0.005(4)        | -0.012(4)       |
| C25A | 0.034(5)        | 0.044(6)        | 0.035(5)        | 0.004(5)        | 0.001(4)        | 0.001(5)        |
| C24  | 0.060(7)        | 0.043(7)        | 0.033(6)        | -0.004(5)       | -0.004(5)       | -0.003(5)       |
| O2A  | 0.060(5)        | 0.039(4)        | 0.035(4)        | -0.005(3)       | -0.022(4)       | -0.005(4)       |
| C2   | 0.035(6)        | 0.028(5)        | 0.036(6)        | 0.003(4)        | -0.006(5)       | -0.008(5)       |
| C31A | 0.031(6)        | 0.033(6)        | 0.034(6)        | -0.004(5)       | -0.001(5)       | -0.003(4)       |
| N4   | 0.033(5)        | 0.035(5)        | 0.031(4)        | 0.004(3)        | -0.002(4)       | -0.002(4)       |
| C22  | 0.060(8)        | 0.039(6)        | 0.040(6)        | 0.011(5)        | -0.009(6)       | 0.005(6)        |
| N2   | 0.045(5)        | 0.028(4)        | 0.026(4)        | 0.005(3)        | 0.001(3)        | -0.005(4)       |
| C21A | 0.026(6)        | 0.032(6)        | 0.041(6)        | -0.004(5)       | 0.002(5)        | -0.001(4)       |
| C3A  | 0.034(6)        | 0.025(5)        | 0.038(6)        | 0.000(4)        | 0.001(5)        | -0.001(5)       |
| C2A  | 0.041(6)        | 0.029(6)        | 0.039(6)        | 0.003(5)        | 0.006(5)        | -0.006(4)       |
| N1A  | 0.035(5)        | 0.030(4)        | 0.022(4)        | 0.000(3)        | -0.001(3)       | 0.004(3)        |
| O4S  | 0.080(6)        | 0.075(6)        | 0.048(5)        | -0.011(4)       | -0.005(4)       | -0.004(5)       |
| C31  | 0.037(6)        | 0.023(6)        | 0.050(7)        | 0.003(4)        | 0.003(5)        | 0.003(4)        |
| C35A | 0.039(6)        | 0.033(5)        | 0.039(6)        | 0.000(5)        | -0.002(5)       | 0.007(4)        |
| N1   | 0.045(5)        | 0.018(4)        | 0.026(4)        | 0.000(3)        | 0.006(4)        | 0.000(4)        |
| N4A  | 0.034(5)        | 0.030(4)        | 0.027(4)        | -0.005(3)       | -0.001(4)       | 0.002(4)        |
| C26  | 0.055(7)        | 0.043(6)        | 0.034(6)        | -0.002(5)       | 0.002(5)        | 0.006(5)        |
| N2A  | 0.034(5)        | 0.025(4)        | 0.037(5)        | 0.003(4)        | 0.002(4)        | -0.001(4)       |
| C15A | 0.052(6)        | 0.029(5)        | 0.038(6)        | 0.004(5)        | -0.007(6)       | -0.002(4)       |
| C33A | 0.066(7)        | 0.032(6)        | 0.059(8)        | 0.003(6)        | 0.002(7)        | 0.007(5)        |

|      | U <sub>11</sub> | U <sub>22</sub> | U <sub>33</sub> | U <sub>23</sub> | U <sub>13</sub> | U <sub>12</sub> |
|------|-----------------|-----------------|-----------------|-----------------|-----------------|-----------------|
| C3   | 0.037(6)        | 0.029(5)        | 0.036(6)        | 0.002(5)        | -0.002(5)       | -0.006(4)       |
| C24A | 0.067(8)        | 0.043(6)        | 0.032(6)        | -0.004(5)       | -0.007(6)       | 0.014(6)        |
| O1S  | 0.080(6)        | 0.050(5)        | 0.077(6)        | 0.010(4)        | -0.008(5)       | -0.007(4)       |
| C13  | 0.058(7)        | 0.032(6)        | 0.041(6)        | -0.013(5)       | -0.004(5)       | 0.003(5)        |
| C12  | 0.053(6)        | 0.028(5)        | 0.032(6)        | 0.001(4)        | -0.005(5)       | 0.002(4)        |
| C23A | 0.063(8)        | 0.055(8)        | 0.038(7)        | -0.014(6)       | 0.000(6)        | 0.014(6)        |
| C22A | 0.055(7)        | 0.029(6)        | 0.052(7)        | -0.014(5)       | 0.001(6)        | 0.004(5)        |
| C11A | 0.031(5)        | 0.027(5)        | 0.028(5)        | 0.001(4)        | 0.003(5)        | -0.006(4)       |
| O2   | 0.074(6)        | 0.035(4)        | 0.044(5)        | 0.008(3)        | -0.018(4)       | 0.005(4)        |
| O3S  | 0.063(5)        | 0.059(5)        | 0.062(5)        | -0.006(4)       | 0.010(4)        | -0.001(4)       |
| C21  | 0.031(6)        | 0.037(6)        | 0.040(6)        | 0.006(5)        | 0.001(5)        | 0.002(5)        |
| C23  | 0.078(9)        | 0.062(8)        | 0.022(6)        | 0.008(5)        | 0.007(6)        | -0.012(7)       |
| C11  | 0.028(6)        | 0.028(5)        | 0.032(6)        | -0.001(4)       | 0.005(5)        | -0.003(4)       |
| O5S  | 0.092(7)        | 0.089(7)        | 0.082(7)        | -0.022(6)       | -0.011(6)       | 0.021(6)        |
| C16  | 0.040(6)        | 0.028(5)        | 0.030(5)        | -0.004(4)       | 0.010(5)        | -0.002(4)       |
| C13A | 0.053(7)        | 0.047(6)        | 0.030(6)        | 0.007(5)        | 0.002(5)        | 0.007(6)        |
| O6S  | 0.066(7)        | 0.138(9)        | 0.089(7)        | 0.044(7)        | -0.001(5)       | 0.011(6)        |
| C32  | 0.060(7)        | 0.028(6)        | 0.049(7)        | 0.006(5)        | -0.001(6)       | 0.012(5)        |
| C35  | 0.038(6)        | 0.025(5)        | 0.048(7)        | -0.005(5)       | -0.002(5)       | 0.001(4)        |
| C14A | 0.047(7)        | 0.050(7)        | 0.049(7)        | 0.015(6)        | -0.004(6)       | -0.005(6)       |
| C14  | 0.066(8)        | 0.045(6)        | 0.026(6)        | -0.008(5)       | -0.007(5)       | 0.006(6)        |
| C34A | 0.057(7)        | 0.031(6)        | 0.054(7)        | 0.009(5)        | -0.011(6)       | 0.017(5)        |
| C33  | 0.074(8)        | 0.019(5)        | 0.074(8)        | -0.002(6)       | 0.002(7)        | 0.007(5)        |
| C12A | 0.056(7)        | 0.041(6)        | 0.026(5)        | -0.003(4)       | 0.002(5)        | -0.004(5)       |
| C34  | 0.058(8)        | 0.035(6)        | 0.074(9)        | -0.018(6)       | 0.006(7)        | -0.009(5)       |
| C36A | 0.046(7)        | 0.039(6)        | 0.049(6)        | 0.002(5)        | -0.013(5)       | 0.005(5)        |
| C32A | 0.059(7)        | 0.025(6)        | 0.049(7)        | -0.004(5)       | -0.002(6)       | 0.001(5)        |
| O2S  | 0.093(8)        | 0.156(10)       | 0.103(9)        | 0.029(8)        | -0.033(7)       | 0.008(8)        |
| C16A | 0.033(6)        | 0.036(6)        | 0.023(5)        | -0.004(4)       | 0.000(5)        | -0.003(5)       |
| C26A | 0.044(7)        | 0.061(8)        | 0.043(7)        | 0.005(5)        | 0.011(5)        | 0.004(6)        |
| C36  | 0.058(7)        | 0.046(6)        | 0.049(7)        | -0.009(5)       | -0.007(6)       | -0.004(6)       |
| C15  | 0.064(7)        | 0.034(6)        | 0.028(5)        | 0.004(4)        | -0.001(5)       | -0.001(5)       |
| C25  | 0.038(5)        | 0.043(6)        | 0.031(5)        | -0.004(5)       | -0.004(4)       | -0.008(6)       |

**Table S8. Hydrogen atomic coordinates and isotropic atomic displacement parameters (Å<sup>2</sup>) for CS\_MeBPCH.**

|      | x/a     | y/b    | z/c     | U(eq) |
|------|---------|--------|---------|-------|
| H24A | 0.2472  | 0.7611 | -0.0183 | 0.054 |
| H22A | 0.1007  | 0.9084 | 0.0614  | 0.056 |
| H26A | 0.3037  | 0.6731 | 0.0323  | 0.066 |
| H26B | 0.3585  | 0.6850 | 0.0957  | 0.066 |
| H26C | 0.1858  | 0.6593 | 0.0833  | 0.066 |
| H15A | 0.6190  | 0.9246 | 0.2104  | 0.048 |
| H15B | 0.4608  | 0.8880 | 0.1975  | 0.048 |
| H33A | 0.6734  | 0.4864 | 0.3027  | 0.063 |
| H24B | 0.5846  | 0.7868 | 0.5239  | 0.057 |
| H13A | 0.2119  | 0.9446 | 0.3740  | 0.052 |
| H13B | 0.0417  | 0.9157 | 0.3640  | 0.052 |
| H12A | 0.1548  | 0.9360 | 0.2747  | 0.045 |
| H12B | 0.3113  | 0.8997 | 0.2905  | 0.045 |
| H23A | 0.6764  | 0.8827 | 0.5150  | 0.062 |
| H22B | 0.7055  | 0.9244 | 0.4236  | 0.055 |
| H11A | 0.4684  | 0.7787 | 0.1926  | 0.034 |
| H23B | 0.1665  | 0.8598 | -0.0225 | 0.065 |
| H11B | 0.0009  | 0.8463 | 0.2820  | 0.035 |
| H16A | 0.3046  | 0.7950 | 0.3063  | 0.039 |
| H13C | 0.6109  | 0.8309 | 0.0597  | 0.052 |
| H13D | 0.4535  | 0.8281 | 0.0969  | 0.052 |
| H32A | 0.2076  | 0.5609 | 0.3022  | 0.055 |
| H14A | 0.5626  | 0.9221 | 0.1099  | 0.058 |
| H14B | 0.7331  | 0.8950 | 0.1235  | 0.058 |
| H14C | 0.1649  | 0.8613 | 0.4344  | 0.055 |
| H14D | 0.3217  | 0.8535 | 0.3974  | 0.055 |
| H34A | 0.8039  | 0.5321 | 0.3780  | 0.057 |
| H33B | 0.1121  | 0.4891 | 0.2357  | 0.067 |
| H12C | 0.5927  | 0.7387 | 0.1117  | 0.049 |
| H12D | 0.7519  | 0.7737 | 0.1267  | 0.049 |
| H34B | -0.0225 | 0.5242 | 0.1545  | 0.067 |
| H36A | 0.9060  | 0.6166 | 0.4245  | 0.067 |
| H36B | 0.9495  | 0.6690 | 0.3822  | 0.067 |
| H36C | 0.7958  | 0.6738 | 0.4212  | 0.067 |
| H32B | 0.5755  | 0.5451 | 0.2284  | 0.053 |
| H16B | 0.7665  | 0.8348 | 0.2129  | 0.037 |
| H26D | 0.5026  | 0.6938 | 0.4837  | 0.074 |

|      | <b>x/a</b> | <b>y/b</b> | <b>z/c</b> | <b>U(eq)</b> |
|------|------------|------------|------------|--------------|
| H26E | 0.4278     | 0.7004     | 0.4223     | 0.074        |
| H26F | 0.6021     | 0.6741     | 0.4297     | 0.074        |
| H36D | -0.1204    | 0.6012     | 0.0947     | 0.077        |
| H36E | -0.1677    | 0.6588     | 0.1298     | 0.077        |
| H36F | -0.0125    | 0.6591     | 0.0913     | 0.077        |
| H15C | 0.1800     | 0.7626     | 0.3922     | 0.051        |
| H15D | 0.0209     | 0.7962     | 0.3741     | 0.051        |

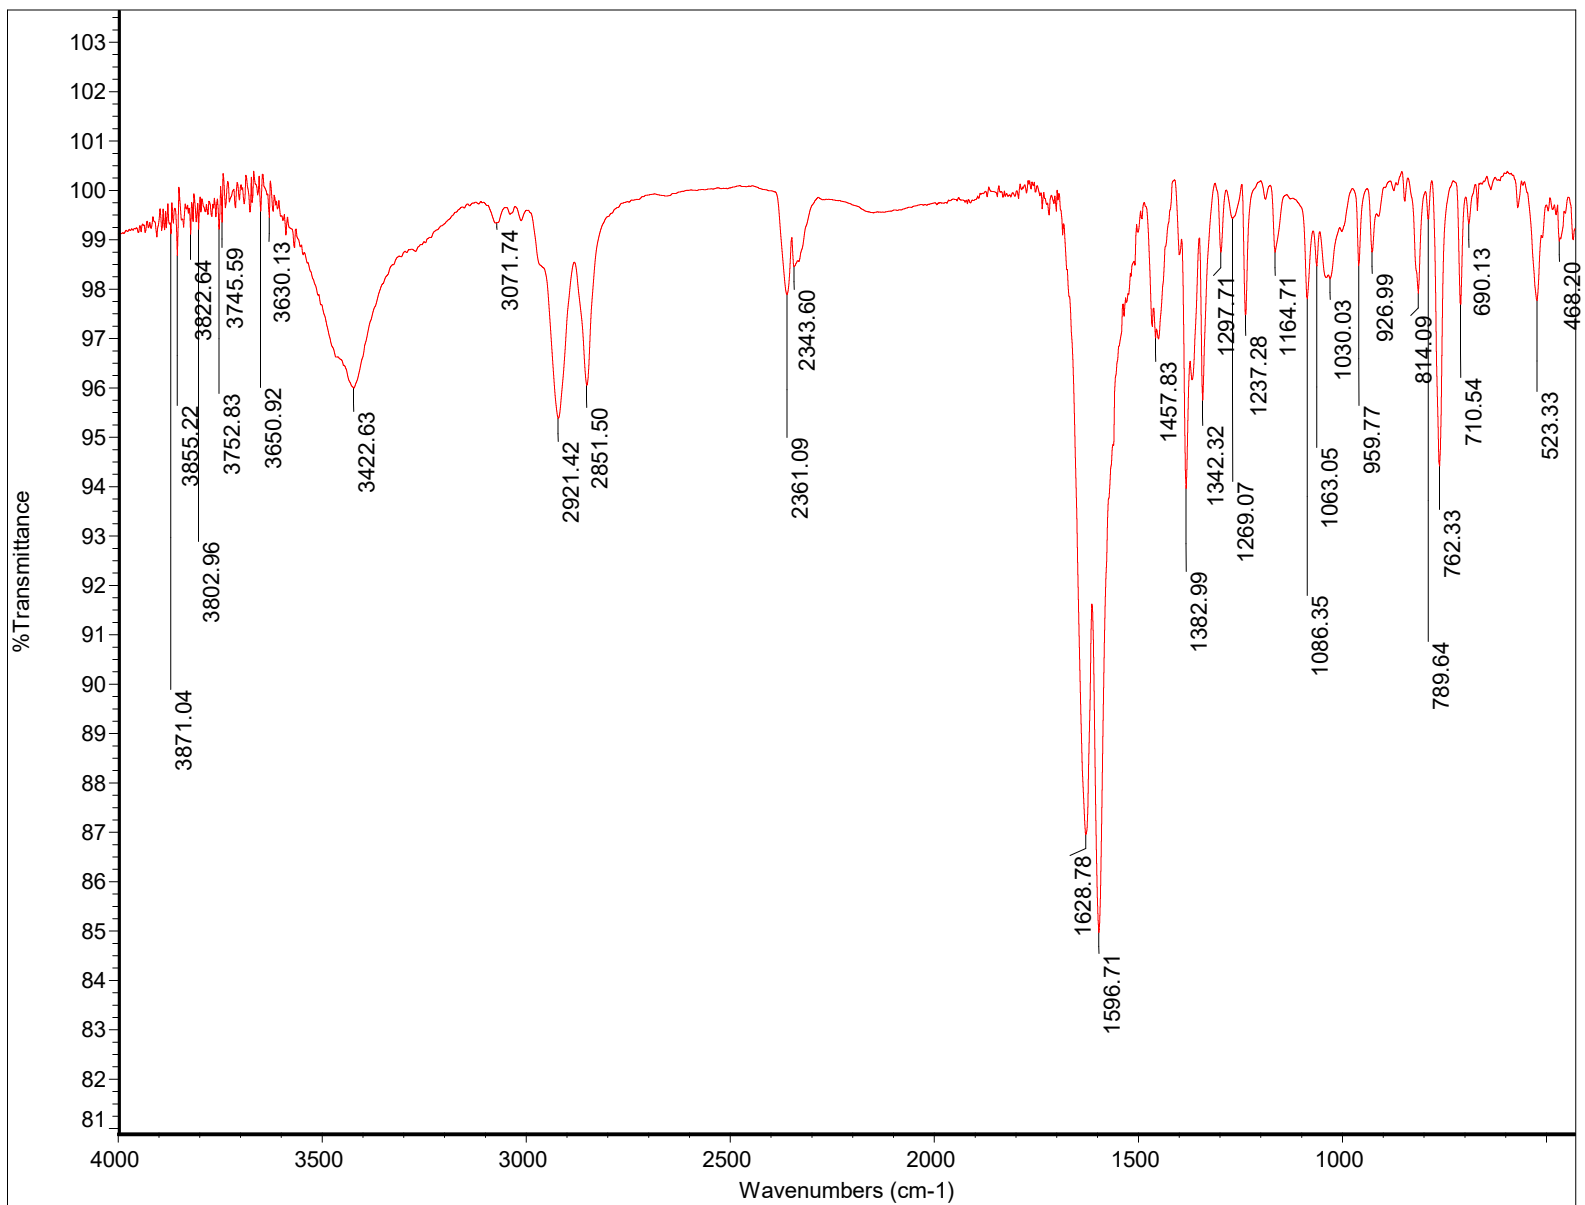

Figure S13: KBr matrix IR spectrum of PtMeBPCH

## Proposed syntheses of PtMeBPCH analogs

**Au(Me-BPCH)** The open shell analog to Pt(Me-BPCH) with a paramagnetic  $d^9$  Au(II) instead of closed shell  $d^8$  Pt(II) would be formed by metallation with Au(III) in the form of auric acid, followed by reduction with the potassium doped graphite reagent. This reaction is best done dilute and at low temperature to diminish disproportionation of the Au(II) product.

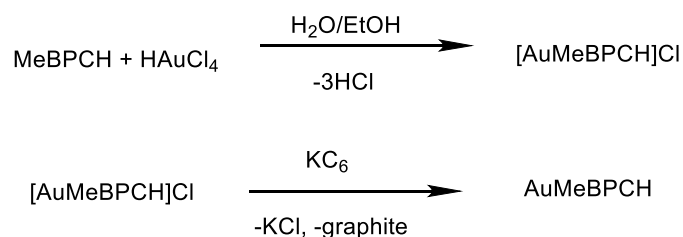

**Pt(CF<sub>3</sub>-BPCH)** The bis trifluoromethyl analog would be most easily prepared by treating 6-trifluoromethylpicolinic acid with one of the enantiomers of 1,2-diaminocyclohexane with the methods described above. If more enhanced helical distortion is sought then the corresponding 6-t-butylpicolinic acid may be another reagent to consider.

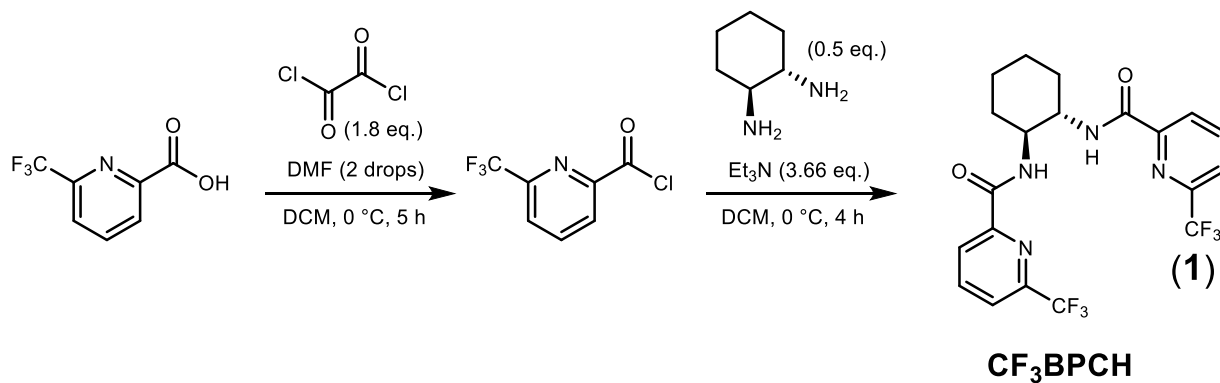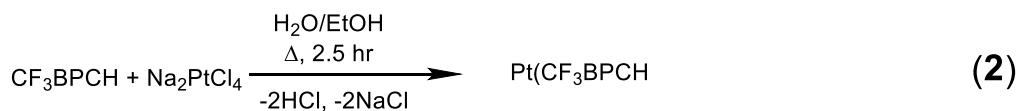



## Computational

### Optimized structure compared to experiment

Figure S14 show the overlay of structures obtained from experimental x-ray diffraction (XRD) data and calculated structure of Pt(Me-BPCH), displaying a good agreement between the two structures, with root mean square deviation (RMSD) of 0.33 Å, or 0.1 Å excluding hydrogens. Cartesian coordinates of both aligned structures are presented in Table S9.

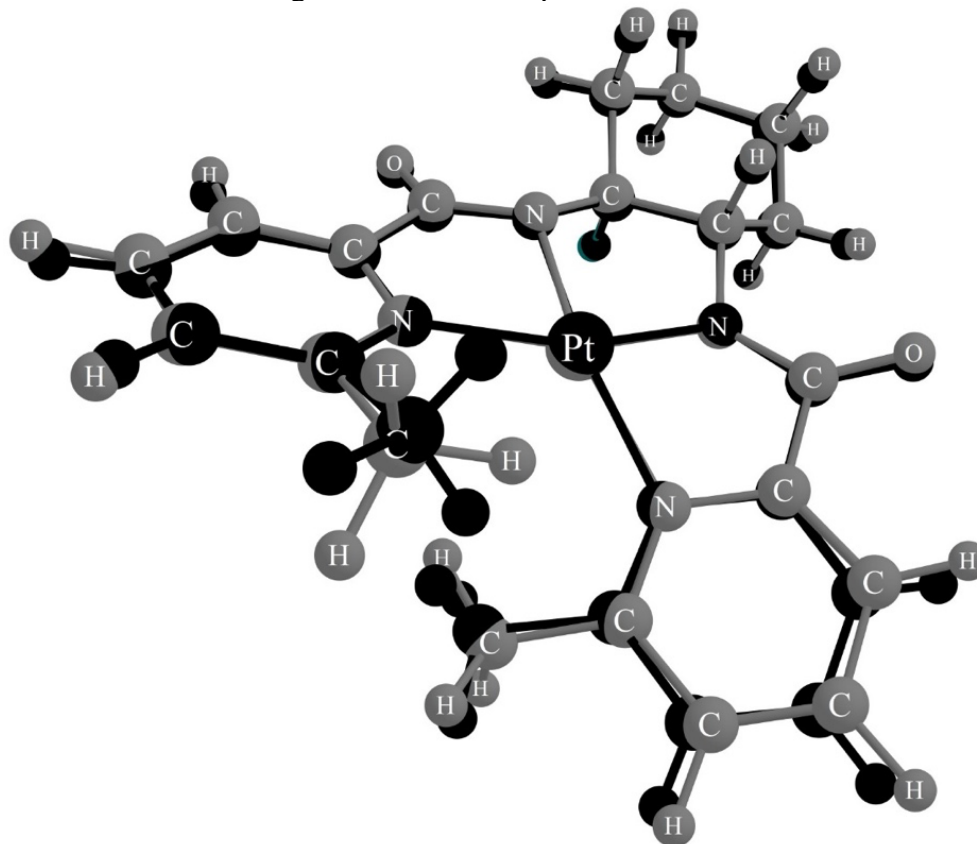

Figure S14: Overlay of XRD (black) and calculated (grey) structures of Pt(Me-BPCH).

Table S9 Coordinates of XRD and Optimized structure of Pt(Me-BPCH)

| Atom | XRD Structure |         |         | Optimized Structure |         |         |
|------|---------------|---------|---------|---------------------|---------|---------|
|      | x             | y       | z       | x                   | y       | z       |
| Pt   | 0.0000        | 0.0000  | 0.0000  | 0.0000              | 0.0000  | 0.0000  |
| O    | 0.6522        | -3.9056 | 0.5522  | 0.7291              | -3.8695 | 0.5365  |
| N    | 0.2356        | 2.0481  | -0.1298 | 0.3269              | 2.0724  | -0.1531 |
| C    | -0.7242       | -0.7852 | 4.2347  | -0.5207             | -0.8649 | 4.3018  |
| H    | -0.9898       | -0.3448 | 5.0096  | -0.8292             | -0.3691 | 5.2118  |
| C    | 0.2361        | -2.7264 | 0.6128  | 0.2978              | -2.7283 | 0.6071  |
| N    | -0.2303       | -0.7064 | 1.9362  | -0.1818             | -0.7400 | 1.9607  |
| C    | -0.0218       | -2.7476 | 3.1410  | 0.2077              | -2.7946 | 3.1164  |

|   |         |         |         |         |         |         |
|---|---------|---------|---------|---------|---------|---------|
| H | 0.1750  | -3.6563 | 3.1611  | 0.4888  | -3.8345 | 3.0363  |
| N | -0.1683 | 0.2269  | -1.9359 | -0.0540 | 0.2106  | -1.9546 |
| C | -0.2297 | 2.4721  | -1.3439 | -0.0805 | 2.4871  | -1.3740 |
| N | -0.1026 | -1.9248 | -0.3717 | -0.1329 | -1.9264 | -0.3731 |
| C | -1.2134 | 1.2912  | 2.9476  | -1.1618 | 1.2163  | 3.0711  |
| H | -1.4941 | 1.5896  | 3.8158  | -0.6815 | 1.8697  | 3.7980  |
| H | -0.5271 | 1.8745  | 2.6153  | -1.0922 | 1.6565  | 2.0814  |
| H | -1.9624 | 1.3038  | 2.3473  | -2.2191 | 1.1539  | 3.3327  |
| C | -0.6281 | 1.4088  | -2.3585 | -0.4408 | 1.4155  | -2.3880 |
| C | -0.2740 | -3.6608 | -3.8034 | -0.1439 | -3.7018 | -3.7770 |
| H | 0.6784  | -3.8195 | -3.8968 | 0.9369  | -3.8598 | -3.8470 |
| H | -0.7365 | -4.4435 | -4.1414 | -0.6152 | -4.6065 | -4.1649 |
| C | -0.6029 | -3.5008 | -2.3094 | -0.5159 | -3.5130 | -2.3056 |
| H | -1.5648 | -3.4798 | -2.1858 | -1.6029 | -3.4651 | -2.1900 |
| H | -0.2497 | -4.2558 | -1.8133 | -0.1580 | -4.3470 | -1.7065 |
| O | -1.1723 | 1.6923  | -3.4065 | -0.9629 | 1.7224  | -3.4494 |
| C | 0.0554  | -2.0708 | 1.9547  | 0.1274  | -2.0564 | 1.9583  |
| C | -0.3819 | -2.1154 | 4.2954  | -0.0957 | -2.1776 | 4.3180  |
| H | -0.3955 | -2.5737 | 5.1045  | -0.0377 | -2.7235 | 5.2501  |
| C | 0.0111  | -2.2098 | -1.7877 | 0.0934  | -2.2140 | -1.7920 |
| H | 0.9695  | -2.2566 | -1.9866 | 1.1794  | -2.2634 | -1.9507 |
| C | -0.5368 | -1.0659 | -2.5916 | -0.4474 | -1.0359 | -2.6170 |
| H | -1.5138 | -1.1351 | -2.5594 | -1.5446 | -1.0891 | -2.5975 |
| C | -0.3189 | 3.8159  | -1.6545 | -0.0965 | 3.8154  | -1.7314 |
| H | -0.6979 | 4.0930  | -2.4573 | -0.4630 | 4.0716  | -2.7148 |
| C | 0.8302  | 2.9261  | 0.7300  | 0.8808  | 2.9562  | 0.6882  |
| C | -0.6445 | -2.4942 | -4.6365 | -0.5314 | -2.4976 | -4.6336 |
| H | -1.6105 | -2.4544 | -4.7153 | -1.6225 | -2.4344 | -4.6922 |
| H | -0.2781 | -2.6109 | -5.5271 | -0.1734 | -2.6322 | -5.6556 |
| C | 0.1685  | 4.7436  | -0.7441 | 0.3760  | 4.7509  | -0.8268 |
| H | 0.0764  | 5.6558  | -0.9000 | 0.3734  | 5.8051  | -1.0693 |
| C | 0.8012  | 4.2767  | 0.4127  | 0.8961  | 4.3107  | 0.3731  |
| H | 1.2122  | 4.8859  | 0.9827  | 1.3341  | 5.0046  | 1.0772  |
| C | 1.6666  | 2.4238  | 1.8894  | 1.5633  | 2.4691  | 1.9289  |
| H | 2.0058  | 3.1715  | 2.3869  | 1.2122  | 3.0020  | 2.8114  |
| H | 1.1236  | 1.8778  | 2.4627  | 1.4253  | 1.4014  | 2.0673  |
| H | 2.4002  | 1.9038  | 1.5531  | 2.6341  | 2.6558  | 1.8359  |
| C | -0.1324 | -1.1684 | -4.0517 | 0.0044  | -1.1827 | -4.0650 |
| H | 0.8337  | -1.1280 | -4.1279 | 1.0980  | -1.1702 | -4.0984 |
| H | -0.5073 | -0.4245 | -4.5487 | -0.3522 | -0.3363 | -4.6472 |
| C | -0.6799 | -0.0977 | 3.0479  | -0.5763 | -0.1616 | 3.1033  |

---

## Calculated PV Frequency Shifts

Table S10: Calculated frequencies  $\nu$ , intensities  $I$ , and PV frequency shifts  $\Delta\nu_{0\rightarrow1}^{\text{PV}}$  for vibrational modes between 500 – 2000  $\text{cm}^{-1}$  in Pt(Me-BPCH), based on the harmonic vibrational analysis.

| Mode No. | $\nu$ ( $\text{cm}^{-1}$ ) | $I$ ( $\text{km/mol}$ ) | $\text{C}_2$ irrep | $\Delta\nu_{0\rightarrow1}^{\text{PV}}$ (Hz) | $ \Delta\nu_{0\rightarrow1}^{\text{PV}} /\nu$ ( $10^{-14}$ ) | $\Delta\nu_{\text{quad}}^{\text{PV}}$ (Hz) | $\Delta\nu_{\text{anharm}}^{\text{PV}}$ (Hz) |
|----------|----------------------------|-------------------------|--------------------|----------------------------------------------|--------------------------------------------------------------|--------------------------------------------|----------------------------------------------|
| 34       | 530.7                      | 3.2                     | A                  | 1.52                                         | 9.53                                                         | 1.52                                       | -0.02                                        |
| 35       | 532.3                      | 23.1                    | B                  | -0.13                                        | 0.80                                                         | -0.13                                      | 0.00                                         |
| 36       | 539.4                      | 0.7                     | A                  | 0.47                                         | 2.90                                                         | 0.22                                       | 0.25                                         |
| 37       | 544.2                      | 4.2                     | B                  | 0.22                                         | 1.35                                                         | 0.21                                       | 0.00                                         |
| 38       | 579.9                      | 0.2                     | A                  | -1.03                                        | 5.93                                                         | -0.88                                      | -0.14                                        |
| 39       | 582.7                      | 4.5                     | B                  | -1.52                                        | 8.72                                                         | -1.53                                      | 0.00                                         |
| 40       | 652.5                      | 3.5                     | A                  | -3.45                                        | 17.65                                                        | -3.21                                      | -0.25                                        |
| 41       | 657.6                      | 0.7                     | B                  | -1.04                                        | 5.28                                                         | -1.08                                      | 0.00                                         |
| 42       | 710.4                      | 1.4                     | A                  | 0.63                                         | 2.96                                                         | 0.55                                       | 0.09                                         |
| 43       | 712.0                      | 0.1                     | B                  | -0.07                                        | 0.33                                                         | -0.07                                      | 0.00                                         |
| 44       | 743.9                      | 0.3                     | A                  | 1.91                                         | 8.55                                                         | 1.84                                       | 0.07                                         |
| 45       | 745.0                      | 16.9                    | B                  | 1.61                                         | 7.20                                                         | 1.62                                       | 0.00                                         |
| 46       | 798.2                      | 0.0                     | A                  | -1.79                                        | 7.47                                                         | -1.60                                      | -0.24                                        |
| 47       | 799.3                      | 70.5                    | B                  | 0.42                                         | 1.74                                                         | 0.40                                       | 0.00                                         |
| 48       | 810.1                      | 6.5                     | A                  | 0.34                                         | 1.40                                                         | -0.01                                      | 0.35                                         |
| 49       | 854.2                      | 12.1                    | A                  | 0.90                                         | 3.50                                                         | 0.80                                       | 0.11                                         |
| 50       | 854.2                      | 12.6                    | B                  | 0.91                                         | 3.54                                                         | 0.91                                       | 0.00                                         |
| 51       | 860.4                      | 2.4                     | A                  | -0.37                                        | 1.43                                                         | 0.08                                       | -0.49                                        |
| 52       | 860.9                      | 1.0                     | B                  | 0.16                                         | 0.61                                                         | 0.15                                       | 0.00                                         |
| 53       | 872.1                      | 8.7                     | A                  | 0.19                                         | 0.72                                                         | 0.16                                       | 0.01                                         |
| 54       | 890.1                      | 0.5                     | B                  | -0.24                                        | 0.89                                                         | -0.25                                      | 0.00                                         |
| 55       | 918.8                      | 0.0                     | A                  | 1.14                                         | 4.14                                                         | 1.13                                       | 0.00                                         |
| 56       | 953.1                      | 11.8                    | B                  | 0.19                                         | 0.66                                                         | 0.18                                       | 0.00                                         |
| 57       | 956.0                      | 2.2                     | B                  | 0.06                                         | 0.21                                                         | 0.05                                       | 0.00                                         |
| 58       | 961.5                      | 3.8                     | B                  | 0.18                                         | 0.61                                                         | 0.16                                       | 0.00                                         |
| 59       | 961.6                      | 1.0                     | A                  | 0.32                                         | 1.12                                                         | 0.14                                       | 0.20                                         |
| 60       | 988.9                      | 28.8                    | A                  | 0.46                                         | 1.54                                                         | 0.45                                       | 0.00                                         |
| 61       | 996.6                      | 1.2                     | B                  | -0.11                                        | 0.36                                                         | -0.12                                      | 0.00                                         |
| 62       | 1021.2                     | 0.1                     | A                  | 0.51                                         | 1.66                                                         | 0.48                                       | 0.01                                         |
| 63       | 1023.3                     | 4.0                     | B                  | 0.36                                         | 1.19                                                         | 0.36                                       | 0.00                                         |
| 64       | 1047.5                     | 1.5                     | B                  | 0.43                                         | 1.36                                                         | 0.43                                       | 0.00                                         |
| 65       | 1047.6                     | 0.0                     | A                  | 0.45                                         | 1.44                                                         | 0.46                                       | -0.01                                        |
| 66       | 1058.6                     | 3.0                     | B                  | 1.07                                         | 3.37                                                         | 1.08                                       | 0.00                                         |
| 67       | 1061.2                     | 0.6                     | A                  | 2.06                                         | 6.47                                                         | 1.68                                       | 0.37                                         |
| 68       | 1067.2                     | 7.0                     | B                  | 0.29                                         | 0.91                                                         | 0.28                                       | 0.00                                         |
| 69       | 1068.1                     | 0.8                     | A                  | 0.07                                         | 0.21                                                         | -0.02                                      | 0.08                                         |
| 70       | 1074.9                     | 3.4                     | B                  | 0.07                                         | 0.22                                                         | 0.03                                       | 0.00                                         |
| 71       | 1089.8                     | 0.7                     | A                  | 1.20                                         | 3.68                                                         | 1.31                                       | -0.11                                        |
| 72       | 1097.2                     | 14.1                    | A                  | 0.73                                         | 2.23                                                         | 0.72                                       | 0.02                                         |
| 73       | 1104.3                     | 14.5                    | B                  | 0.37                                         | 1.11                                                         | 0.36                                       | 0.00                                         |

|     |        |       |   |       |      |       |       |
|-----|--------|-------|---|-------|------|-------|-------|
| 74  | 1122.0 | 1.8   | A | 0.10  | 0.30 | 0.29  | -0.19 |
| 75  | 1124.4 | 11.6  | B | 0.08  | 0.24 | 0.06  | 0.00  |
| 76  | 1126.5 | 36.0  | A | 0.64  | 1.88 | 0.61  | 0.02  |
| 77  | 1164.0 | 1.4   | A | 0.08  | 0.22 | 0.01  | 0.06  |
| 78  | 1189.8 | 2.9   | B | -0.18 | 0.51 | -0.20 | 0.00  |
| 79  | 1190.0 | 11.1  | A | -0.17 | 0.48 | -0.24 | 0.05  |
| 80  | 1198.4 | 0.8   | B | 0.36  | 1.00 | 0.35  | 0.00  |
| 81  | 1233.8 | 1.5   | A | -0.15 | 0.39 | -0.14 | -0.01 |
| 82  | 1236.4 | 8.7   | B | -0.45 | 1.22 | -0.46 | 0.00  |
| 83  | 1256.4 | 0.3   | A | -0.12 | 0.32 | -0.16 | 0.03  |
| 84  | 1276.4 | 10.0  | A | 0.04  | 0.09 | 0.06  | -0.04 |
| 85  | 1280.9 | 19.1  | B | 0.12  | 0.32 | 0.11  | 0.00  |
| 86  | 1289.3 | 1.6   | B | 0.13  | 0.33 | 0.13  | 0.00  |
| 87  | 1290.7 | 4.7   | A | -0.22 | 0.58 | -0.23 | 0.00  |
| 88  | 1313.4 | 13.0  | B | -0.80 | 2.03 | -0.82 | 0.00  |
| 89  | 1313.6 | 17.8  | A | 0.73  | 1.84 | 0.61  | 0.13  |
| 90  | 1327.1 | 0.2   | B | 0.42  | 1.06 | 0.42  | 0.00  |
| 91  | 1348.4 | 24.1  | B | 0.43  | 1.08 | 0.42  | 0.00  |
| 92  | 1358.1 | 4.4   | A | 0.26  | 0.65 | 0.24  | 0.01  |
| 93  | 1380.9 | 2.6   | B | 0.05  | 0.11 | 0.03  | 0.00  |
| 94  | 1382.3 | 5.9   | A | 0.34  | 0.82 | 0.32  | 0.02  |
| 95  | 1391.8 | 0.0   | A | 0.09  | 0.21 | 0.11  | -0.03 |
| 96  | 1396.5 | 123.6 | B | 1.18  | 2.83 | 1.17  | 0.00  |
| 97  | 1411.9 | 0.1   | A | 0.52  | 1.23 | 0.53  | -0.02 |
| 98  | 1417.1 | 19.5  | B | 0.06  | 0.14 | 0.03  | 0.00  |
| 99  | 1418.9 | 42.0  | A | 0.39  | 0.92 | -0.17 | 0.57  |
| 100 | 1427.2 | 53.3  | B | 1.21  | 2.84 | 1.22  | 0.00  |
| 101 | 1428.9 | 204.3 | A | 1.21  | 2.83 | 0.68  | 0.53  |
| 102 | 1455.4 | 10.4  | B | 0.93  | 2.13 | 0.92  | 0.00  |
| 103 | 1458.8 | 13.9  | A | 2.12  | 4.85 | 1.83  | 0.29  |
| 104 | 1487.0 | 12.8  | B | 0.41  | 0.92 | 0.40  | 0.00  |
| 105 | 1490.1 | 0.4   | A | 0.19  | 0.43 | 0.17  | 0.00  |
| 106 | 1496.6 | 3.6   | B | 0.27  | 0.60 | 0.26  | 0.00  |
| 107 | 1496.9 | 1.0   | B | 0.37  | 0.82 | 0.36  | 0.00  |
| 108 | 1499.1 | 0.5   | A | -0.02 | 0.04 | -0.03 | 0.00  |
| 109 | 1508.4 | 14.8  | A | 1.00  | 2.21 | 0.73  | 0.25  |
| 110 | 1510.0 | 11.7  | B | 0.02  | 0.05 | 0.02  | 0.00  |
| 111 | 1517.8 | 6.1   | A | -0.02 | 0.05 | -0.02 | -0.02 |
| 112 | 1520.6 | 13.5  | B | 0.84  | 1.84 | 0.84  | 0.00  |
| 113 | 1520.7 | 14.8  | A | 0.27  | 0.59 | 0.23  | 0.03  |
| 114 | 1648.3 | 5.1   | B | 0.61  | 1.23 | 0.60  | 0.00  |
| 115 | 1649.9 | 34.5  | A | 0.54  | 1.10 | 0.59  | -0.04 |
| 116 | 1681.8 | 193.3 | B | 0.68  | 1.35 | 0.68  | 0.00  |
| 117 | 1682.3 | 0.1   | A | 0.52  | 1.03 | 0.73  | -0.21 |
| 118 | 1751.6 | 926.2 | B | -1.49 | 2.84 | -1.52 | 0.00  |
| 119 | 1757.8 | 133.8 | A | 0.97  | 1.84 | 0.01  | 0.99  |

Table S11: Calculated frequencies  $\nu$ , intensities  $I$ , and PV frequency shifts  $\Delta\nu_{0\rightarrow 1}^{\text{PV}}$  for vibrational modes between 500 – 2000  $\text{cm}^{-1}$  in Au(Me-BPCH), based on the harmonic vibrational analysis.

| Mode No. | $\nu$ ( $\text{cm}^{-1}$ ) | $I$ ( $\text{km/mol}$ ) | $\text{C}_2$ irrep | $\Delta\nu_{0\rightarrow 1}^{\text{PV}}$ (Hz) | $ \Delta\nu_{0\rightarrow 1}^{\text{PV}} /\nu$ ( $10^{-14}$ ) | $\Delta\nu_{\text{quad}}^{\text{PV}}$ (Hz) | $\Delta\nu_{\text{anharm}}^{\text{PV}}$ (Hz) |
|----------|----------------------------|-------------------------|--------------------|-----------------------------------------------|---------------------------------------------------------------|--------------------------------------------|----------------------------------------------|
| 34       | 512.7                      | 20.2                    | B                  | -0.79                                         | 5.13                                                          | -0.79                                      | 0.00                                         |
| 35       | 518.0                      | 0.9                     | A                  | 2.93                                          | 18.85                                                         | 3.22                                       | -0.31                                        |
| 36       | 537.0                      | 1.9                     | A                  | -0.20                                         | 1.26                                                          | -0.22                                      | 0.04                                         |
| 37       | 547.0                      | 6.3                     | B                  | 0.04                                          | 0.26                                                          | 0.04                                       | 0.00                                         |
| 38       | 568.3                      | 0.8                     | B                  | 0.15                                          | 0.90                                                          | 0.16                                       | 0.00                                         |
| 39       | 571.0                      | 0.0                     | A                  | 0.35                                          | 2.07                                                          | 0.33                                       | 0.02                                         |
| 40       | 636.2                      | 2.0                     | A                  | 2.10                                          | 11.03                                                         | 2.02                                       | 0.07                                         |
| 41       | 647.4                      | 1.5                     | B                  | -0.53                                         | 2.72                                                          | -0.53                                      | 0.00                                         |
| 42       | 694.2                      | 21.2                    | B                  | 2.66                                          | 12.77                                                         | 2.66                                       | 0.00                                         |
| 43       | 702.2                      | 6.1                     | A                  | 0.69                                          | 3.28                                                          | 0.64                                       | 0.05                                         |
| 44       | 741.3                      | 0.0                     | A                  | -0.04                                         | 0.17                                                          | 0.00                                       | -0.02                                        |
| 45       | 741.7                      | 13.2                    | B                  | 0.27                                          | 1.21                                                          | 0.28                                       | 0.00                                         |
| 46       | 795.6                      | 0.1                     | A                  | 0.88                                          | 3.70                                                          | 1.04                                       | -0.09                                        |
| 47       | 797.0                      | 63.4                    | B                  | 0.01                                          | 0.05                                                          | 0.02                                       | 0.00                                         |
| 48       | 804.1                      | 6.7                     | A                  | 0.19                                          | 0.78                                                          | 0.29                                       | -0.08                                        |
| 49       | 852.5                      | 12.1                    | A                  | 0.13                                          | 0.49                                                          | 0.24                                       | -0.11                                        |
| 50       | 855.1                      | 4.1                     | B                  | 0.66                                          | 2.57                                                          | 0.66                                       | 0.00                                         |
| 51       | 857.8                      | 18.9                    | B                  | 0.21                                          | 0.82                                                          | 0.21                                       | 0.00                                         |
| 52       | 858.4                      | 3.0                     | A                  | 0.67                                          | 2.60                                                          | 0.72                                       | -0.02                                        |
| 53       | 867.3                      | 6.5                     | A                  | -0.07                                         | 0.25                                                          | 0.08                                       | -0.14                                        |
| 54       | 870.0                      | 2.3                     | B                  | -0.39                                         | 1.48                                                          | -0.39                                      | 0.00                                         |
| 55       | 918.9                      | 0.1                     | A                  | -0.11                                         | 0.38                                                          | -0.10                                      | -0.01                                        |
| 56       | 942.8                      | 3.2                     | B                  | 0.15                                          | 0.53                                                          | 0.15                                       | 0.00                                         |
| 57       | 954.1                      | 15.0                    | B                  | -0.17                                         | 0.58                                                          | -0.17                                      | 0.00                                         |
| 58       | 963.3                      | 2.4                     | B                  | -0.08                                         | 0.27                                                          | -0.08                                      | 0.00                                         |
| 59       | 963.4                      | 0.2                     | A                  | 0.24                                          | 0.84                                                          | 0.21                                       | 0.05                                         |
| 60       | 963.9                      | 28.5                    | A                  | 0.82                                          | 2.84                                                          | 0.81                                       | 0.00                                         |
| 61       | 985.4                      | 1.6                     | B                  | 0.11                                          | 0.36                                                          | 0.11                                       | 0.00                                         |
| 62       | 1019.8                     | 0.2                     | A                  | 0.03                                          | 0.10                                                          | 0.03                                       | 0.00                                         |
| 63       | 1020.5                     | 12.0                    | B                  | 0.94                                          | 3.07                                                          | 0.94                                       | 0.00                                         |
| 64       | 1039.1                     | 24.3                    | B                  | 3.45                                          | 11.09                                                         | 3.50                                       | 0.00                                         |
| 65       | 1044.3                     | 3.1                     | A                  | 2.19                                          | 7.01                                                          | 1.83                                       | 0.36                                         |
| 66       | 1051.9                     | 0.7                     | B                  | 1.02                                          | 3.24                                                          | 1.05                                       | 0.00                                         |
| 67       | 1052.1                     | 0.0                     | A                  | 0.81                                          | 2.56                                                          | 0.85                                       | 0.00                                         |
| 68       | 1068.5                     | 5.7                     | B                  | 0.14                                          | 0.45                                                          | 0.14                                       | 0.00                                         |
| 69       | 1073.6                     | 5.5                     | B                  | -0.16                                         | 0.49                                                          | -0.16                                      | 0.00                                         |
| 70       | 1074.3                     | 0.7                     | A                  | 0.02                                          | 0.06                                                          | 0.00                                       | 0.00                                         |
| 71       | 1083.0                     | 9.4                     | A                  | -0.07                                         | 0.22                                                          | -0.54                                      | 0.61                                         |
| 72       | 1088.0                     | 0.2                     | A                  | 0.00                                          | 0.01                                                          | 0.05                                       | -0.05                                        |
| 73       | 1101.1                     | 27.3                    | B                  | -1.01                                         | 3.05                                                          | -1.01                                      | 0.00                                         |
| 74       | 1111.4                     | 0.3                     | A                  | 0.07                                          | 0.20                                                          | 0.10                                       | -0.03                                        |

|     |        |       |   |       |      |       |       |
|-----|--------|-------|---|-------|------|-------|-------|
| 75  | 1119.5 | 18.9  | B | 0.28  | 0.85 | 0.29  | 0.00  |
| 76  | 1120.2 | 13.0  | A | 0.30  | 0.89 | 0.32  | -0.02 |
| 77  | 1162.9 | 1.7   | A | -0.11 | 0.31 | -0.11 | 0.00  |
| 78  | 1179.3 | 1.1   | B | 0.04  | 0.11 | 0.03  | 0.00  |
| 79  | 1188.6 | 2.1   | B | -0.12 | 0.34 | -0.12 | 0.00  |
| 80  | 1188.7 | 13.6  | A | -0.09 | 0.25 | -0.09 | 0.00  |
| 81  | 1231.4 | 1.4   | A | -0.20 | 0.53 | -0.20 | 0.00  |
| 82  | 1237.2 | 3.9   | B | -0.57 | 1.55 | -0.57 | 0.00  |
| 83  | 1251.9 | 1.7   | A | -0.16 | 0.44 | -0.17 | 0.00  |
| 84  | 1276.1 | 9.4   | A | 0.01  | 0.03 | 0.00  | 0.02  |
| 85  | 1281.7 | 19.5  | B | 0.15  | 0.38 | 0.14  | 0.00  |
| 86  | 1291.2 | 1.2   | B | -0.04 | 0.10 | -0.04 | 0.00  |
| 87  | 1291.9 | 8.7   | A | 0.07  | 0.18 | 0.06  | 0.01  |
| 88  | 1311.0 | 15.3  | B | -0.79 | 2.01 | -0.79 | 0.00  |
| 89  | 1311.8 | 24.9  | A | -1.48 | 3.77 | -1.29 | -0.23 |
| 90  | 1325.1 | 2.3   | B | 0.07  | 0.17 | 0.07  | 0.00  |
| 91  | 1347.9 | 21.3  | B | 0.69  | 1.70 | 0.69  | 0.00  |
| 92  | 1357.5 | 3.7   | A | 0.19  | 0.46 | 0.19  | -0.01 |
| 93  | 1372.6 | 0.0   | A | -0.24 | 0.57 | -0.25 | 0.00  |
| 94  | 1381.3 | 4.4   | B | -0.07 | 0.17 | -0.07 | 0.00  |
| 95  | 1391.6 | 2.2   | A | -0.03 | 0.07 | 0.00  | -0.04 |
| 96  | 1397.2 | 148.4 | B | -0.24 | 0.58 | -0.19 | 0.00  |
| 97  | 1411.4 | 0.0   | A | 0.59  | 1.39 | 0.61  | -0.02 |
| 98  | 1414.4 | 136.8 | B | -1.94 | 4.58 | -1.94 | 0.00  |
| 99  | 1419.4 | 80.6  | A | 0.43  | 1.01 | 0.14  | 0.30  |
| 100 | 1428.0 | 210.1 | A | 0.23  | 0.53 | 0.21  | 0.04  |
| 101 | 1428.4 | 12.8  | B | -0.10 | 0.23 | -0.10 | 0.00  |
| 102 | 1454.1 | 62.6  | B | 2.66  | 6.11 | 2.66  | 0.00  |
| 103 | 1459.3 | 32.4  | A | 1.50  | 3.43 | 1.32  | 0.19  |
| 104 | 1483.1 | 13.9  | B | 0.58  | 1.29 | 0.57  | 0.00  |
| 105 | 1496.1 | 4.4   | B | -0.08 | 0.17 | -0.08 | 0.00  |
| 106 | 1497.3 | 0.1   | A | 0.42  | 0.92 | 0.44  | -0.04 |
| 107 | 1498.2 | 0.4   | A | -0.07 | 0.16 | -0.07 | 0.00  |
| 108 | 1498.3 | 1.1   | B | 1.72  | 3.83 | 1.74  | 0.00  |
| 109 | 1507.8 | 20.6  | A | 0.44  | 0.98 | 0.47  | -0.02 |
| 110 | 1508.6 | 11.1  | B | -0.07 | 0.16 | -0.07 | 0.00  |
| 111 | 1514.6 | 6.3   | B | -0.40 | 0.87 | -0.39 | 0.00  |
| 112 | 1516.0 | 31.2  | A | 0.51  | 1.12 | 0.53  | -0.03 |
| 113 | 1516.9 | 3.8   | A | -0.05 | 0.12 | -0.04 | -0.01 |
| 114 | 1653.4 | 7.1   | B | 0.25  | 0.51 | 0.25  | 0.00  |
| 115 | 1654.9 | 62.3  | A | 0.63  | 1.27 | 0.65  | -0.02 |
| 116 | 1672.7 | 282.6 | B | 0.91  | 1.82 | 0.86  | 0.00  |
| 117 | 1673.6 | 0.0   | A | 2.54  | 5.07 | 2.16  | 0.69  |
| 118 | 1730.9 | 858.9 | B | 1.16  | 2.23 | 1.15  | 0.00  |
| 119 | 1741.7 | 76.7  | A | 0.81  | 1.55 | 2.61  | -1.80 |

Table S12: Calculated frequencies  $\nu$ , intensities  $I$ , and PV frequency shifts  $\Delta\nu_{0\rightarrow1}^{\text{PV}}$  for vibrational modes between 500 – 2000  $\text{cm}^{-1}$  in Pt(CF<sub>3</sub>-BPCH), based on the harmonic vibrational analysis.

| Mode No. | $\nu$ ( $\text{cm}^{-1}$ ) | $I$ (km/mol) | C <sub>2</sub> irrep | $\Delta\nu_{0\rightarrow1}^{\text{PV}}$ (Hz) | $ \Delta\nu_{0\rightarrow1}^{\text{PV}} /\nu$ ( $10^{-14}$ ) | $\Delta\nu_{\text{quad}}^{\text{PV}}$ (Hz) | $\Delta\nu_{\text{anharm}}^{\text{PV}}$ (Hz) |
|----------|----------------------------|--------------|----------------------|----------------------------------------------|--------------------------------------------------------------|--------------------------------------------|----------------------------------------------|
| 40       | 523.5                      | 0.1          | A                    | 0.55                                         | 3.49                                                         | 0.57                                       | -0.02                                        |
| 41       | 525.1                      | 5.7          | B                    | 0.17                                         | 1.08                                                         | 0.17                                       | 0.00                                         |
| 42       | 541.9                      | 13.0         | B                    | -1.47                                        | 9.04                                                         | -1.46                                      | 0.00                                         |
| 43       | 544.6                      | 5.4          | A                    | -0.13                                        | 0.77                                                         | -0.24                                      | 0.12                                         |
| 44       | 603.7                      | 5.8          | B                    | 0.06                                         | 0.36                                                         | 0.06                                       | 0.00                                         |
| 45       | 606.4                      | 3.1          | A                    | -0.30                                        | 1.65                                                         | -0.27                                      | -0.03                                        |
| 46       | 614.2                      | 6.1          | A                    | 0.35                                         | 1.88                                                         | 0.32                                       | 0.02                                         |
| 47       | 618.1                      | 2.5          | B                    | 0.38                                         | 2.05                                                         | 0.38                                       | 0.00                                         |
| 48       | 656.6                      | 3.1          | A                    | -2.20                                        | 11.18                                                        | -2.09                                      | -0.12                                        |
| 49       | 662.0                      | 4.0          | B                    | -0.79                                        | 3.99                                                         | -0.78                                      | 0.00                                         |
| 50       | 688.3                      | 16.9         | B                    | -0.61                                        | 2.94                                                         | -0.61                                      | 0.00                                         |
| 51       | 690.1                      | 1.2          | A                    | 0.52                                         | 2.53                                                         | 0.58                                       | -0.06                                        |
| 52       | 734.7                      | 21.3         | A                    | 0.12                                         | 0.53                                                         | -0.16                                      | 0.28                                         |
| 53       | 735.3                      | 7.5          | B                    | -0.36                                        | 1.64                                                         | -0.37                                      | 0.00                                         |
| 54       | 774.2                      | 0.0          | A                    | 1.83                                         | 7.87                                                         | 1.85                                       | -0.04                                        |
| 55       | 774.8                      | 10.4         | B                    | 1.94                                         | 8.35                                                         | 1.96                                       | 0.00                                         |
| 56       | 795.7                      | 0.0          | A                    | -0.97                                        | 4.05                                                         | -0.98                                      | 0.04                                         |
| 57       | 797.0                      | 69.9         | B                    | 0.88                                         | 3.69                                                         | 0.89                                       | 0.00                                         |
| 58       | 810.6                      | 5.1          | A                    | 0.26                                         | 1.08                                                         | 0.15                                       | 0.12                                         |
| 59       | 831.2                      | 3.8          | B                    | 0.20                                         | 0.81                                                         | 0.20                                       | 0.00                                         |
| 60       | 839.8                      | 6.8          | A                    | 0.22                                         | 0.89                                                         | 0.39                                       | -0.17                                        |
| 61       | 863.3                      | 9.4          | A                    | 0.18                                         | 0.71                                                         | 0.09                                       | 0.11                                         |
| 62       | 873.9                      | 27.4         | B                    | 0.82                                         | 3.12                                                         | 0.81                                       | 0.00                                         |
| 63       | 875.7                      | 2.5          | A                    | 0.09                                         | 0.34                                                         | 0.04                                       | 0.06                                         |
| 64       | 883.7                      | 4.2          | B                    | -0.41                                        | 1.55                                                         | -0.42                                      | 0.00                                         |
| 65       | 901.4                      | 0.3          | A                    | 0.66                                         | 2.45                                                         | 0.63                                       | 0.02                                         |
| 66       | 944.3                      | 15.3         | B                    | 0.55                                         | 1.95                                                         | 0.56                                       | 0.00                                         |
| 67       | 955.2                      | 3.0          | B                    | -0.01                                        | 0.02                                                         | -0.01                                      | 0.00                                         |
| 68       | 977.7                      | 0.3          | B                    | 0.26                                         | 0.88                                                         | 0.26                                       | 0.00                                         |
| 69       | 977.8                      | 0.2          | A                    | 0.08                                         | 0.27                                                         | 0.11                                       | -0.10                                        |
| 70       | 987.1                      | 10.2         | A                    | 0.87                                         | 2.93                                                         | 0.86                                       | 0.01                                         |
| 71       | 999.1                      | 1.3          | B                    | 0.02                                         | 0.05                                                         | 0.01                                       | 0.00                                         |
| 72       | 1048.5                     | 8.1          | B                    | 0.74                                         | 2.35                                                         | 0.74                                       | 0.00                                         |
| 73       | 1050.6                     | 0.2          | A                    | 1.38                                         | 4.37                                                         | 1.28                                       | 0.10                                         |
| 74       | 1057.1                     | 1.4          | B                    | 0.32                                         | 1.00                                                         | 0.33                                       | 0.00                                         |
| 75       | 1057.6                     | 0.1          | A                    | 0.58                                         | 1.84                                                         | 0.52                                       | 0.09                                         |
| 76       | 1072.8                     | 2.6          | B                    | 0.06                                         | 0.18                                                         | 0.05                                       | 0.00                                         |
| 77       | 1090.5                     | 3.4          | A                    | 0.58                                         | 1.78                                                         | 0.55                                       | 0.02                                         |
| 78       | 1098.2                     | 22.8         | A                    | 0.61                                         | 1.85                                                         | 0.59                                       | 0.02                                         |
| 79       | 1105.4                     | 11.9         | B                    | 0.32                                         | 0.96                                                         | 0.31                                       | 0.00                                         |
| 80       | 1122.4                     | 46.9         | B                    | 0.22                                         | 0.65                                                         | 0.21                                       | 0.00                                         |

|     |        |       |   |       |      |       |       |
|-----|--------|-------|---|-------|------|-------|-------|
| 81  | 1122.5 | 3.4   | A | 0.07  | 0.20 | 0.24  | -0.18 |
| 82  | 1126.5 | 60.2  | A | 0.50  | 1.48 | 0.59  | -0.07 |
| 83  | 1146.6 | 35.9  | A | 0.95  | 2.77 | 0.97  | -0.02 |
| 84  | 1148.2 | 79.6  | B | 0.25  | 0.73 | 0.25  | 0.00  |
| 85  | 1164.2 | 412.8 | B | 0.05  | 0.14 | 0.05  | 0.00  |
| 86  | 1164.7 | 2.7   | A | 0.07  | 0.19 | 0.00  | 0.07  |
| 87  | 1188.4 | 60.9  | A | 0.26  | 0.73 | 0.07  | 0.20  |
| 88  | 1195.9 | 30.5  | B | 0.07  | 0.19 | 0.06  | 0.00  |
| 89  | 1197.5 | 59.9  | A | -0.06 | 0.17 | -0.10 | 0.02  |
| 90  | 1199.9 | 12.4  | B | 0.37  | 1.02 | 0.36  | 0.00  |
| 91  | 1219.7 | 127.9 | B | -0.05 | 0.14 | -0.05 | 0.00  |
| 92  | 1230.2 | 204.3 | A | 0.04  | 0.11 | 0.10  | -0.05 |
| 93  | 1237.7 | 85.4  | A | 0.05  | 0.14 | 0.05  | 0.00  |
| 94  | 1240.4 | 56.3  | B | -0.18 | 0.50 | -0.19 | 0.00  |
| 95  | 1259.3 | 0.4   | A | 0.03  | 0.09 | -0.08 | 0.09  |
| 96  | 1276.3 | 9.8   | A | 0.08  | 0.22 | 0.11  | -0.05 |
| 97  | 1281.0 | 14.2  | B | 0.17  | 0.44 | 0.17  | 0.00  |
| 98  | 1310.4 | 66.2  | A | 0.18  | 0.45 | 0.45  | -0.27 |
| 99  | 1310.6 | 12.9  | B | -1.14 | 2.90 | -1.18 | 0.00  |
| 100 | 1323.8 | 0.4   | B | 0.41  | 1.03 | 0.40  | 0.00  |
| 101 | 1348.0 | 15.8  | B | 0.26  | 0.65 | 0.26  | 0.00  |
| 102 | 1351.0 | 104.2 | A | 0.36  | 0.90 | 0.11  | 0.25  |
| 103 | 1352.4 | 111.7 | B | 0.39  | 0.96 | 0.38  | 0.00  |
| 104 | 1359.0 | 11.4  | A | 0.27  | 0.67 | 0.27  | 0.00  |
| 105 | 1381.3 | 2.9   | B | 0.05  | 0.13 | 0.05  | 0.00  |
| 106 | 1384.8 | 2.8   | A | 0.29  | 0.71 | 0.29  | 0.00  |
| 107 | 1393.2 | 0.1   | A | 0.12  | 0.28 | 0.12  | -0.01 |
| 108 | 1401.8 | 169.1 | B | 0.87  | 2.08 | 0.88  | 0.00  |
| 109 | 1415.0 | 3.1   | A | 0.52  | 1.22 | 0.58  | -0.06 |
| 110 | 1428.7 | 187.0 | B | 2.23  | 5.21 | 2.21  | 0.00  |
| 111 | 1431.8 | 205.8 | A | 1.80  | 4.20 | 0.24  | 1.56  |
| 112 | 1479.6 | 3.5   | B | 1.74  | 3.92 | 1.76  | 0.00  |
| 113 | 1480.5 | 6.3   | A | 3.24  | 7.31 | 2.71  | 0.53  |
| 114 | 1496.8 | 4.7   | B | -0.01 | 0.01 | -0.01 | 0.00  |
| 115 | 1499.2 | 0.6   | A | 0.00  | 0.00 | 0.00  | -0.01 |
| 116 | 1510.0 | 12.3  | B | 0.05  | 0.12 | 0.05  | 0.00  |
| 117 | 1517.8 | 6.1   | A | 0.01  | 0.02 | 0.02  | -0.01 |
| 118 | 1519.1 | 1.0   | A | 0.44  | 0.97 | 0.37  | 0.08  |
| 119 | 1519.7 | 7.5   | B | 0.45  | 0.98 | 0.44  | 0.00  |
| 120 | 1650.5 | 0.5   | B | 0.38  | 0.77 | 0.39  | 0.00  |
| 121 | 1651.0 | 4.5   | A | 0.57  | 1.14 | 0.45  | 0.13  |
| 122 | 1680.9 | 127.9 | B | 0.61  | 1.21 | 0.61  | 0.00  |
| 123 | 1681.1 | 2.5   | A | 0.80  | 1.58 | 0.85  | -0.06 |
| 124 | 1755.9 | 927.0 | B | -1.47 | 2.80 | -1.49 | 0.00  |
| 125 | 1762.2 | 121.0 | A | 1.20  | 2.28 | 0.30  | 0.91  |



## Vibrational modes overlaps

Table S13: Identification of related vibrational modes between 500–2000  $\text{cm}^{-1}$  in the three derivatives. Mode displacement vector overlap with Pt(Me-BPCH) is given in percent for Au(Me-BPCH) and Pt(CF<sub>3</sub>-BPCH). Only modes with dominant overlaps over 75% are shown.

| Pt(Me-BPCH)<br>mode # | Au(Me-BPCH)<br>mode # and overlap | Pt(CF <sub>3</sub> -BPCH)<br>mode # and overlap |
|-----------------------|-----------------------------------|-------------------------------------------------|
| 34                    | 36 81%                            |                                                 |
| 35                    | 34 83%                            |                                                 |
| 37                    | 37 93%                            |                                                 |
| 38                    | 39 97%                            |                                                 |
| 39                    | 38 93%                            |                                                 |
| 40                    | 40 98%                            | 48 83%                                          |
| 41                    | 41 98%                            | 49 91%                                          |
| 42                    | 43 95%                            |                                                 |
| 43                    | 42 93%                            |                                                 |
| 44                    | 44 95%                            |                                                 |
| 45                    | 45 95%                            |                                                 |
| 46                    | 46 99%                            | 56 95%                                          |
| 47                    | 47 100%                           | 57 95%                                          |
| 48                    | 48 99%                            | 58 96%                                          |
| 49                    | 52 84%                            | 63 81%                                          |
| 50                    | 51 94%                            | 62 73%                                          |
| 51                    | 53 80%                            | 61 90%                                          |
| 54                    | 54 89%                            | 64 91%                                          |
| 55                    | 55 99%                            | 65 88%                                          |
| 56                    | 57 86%                            | 67 83%                                          |
| 58                    | 58 99%                            | 68 94%                                          |
| 59                    | 59 99%                            | 69 93%                                          |
| 60                    | 60 92%                            |                                                 |
| 61                    | 61 82%                            |                                                 |
| 62                    | 62 93%                            |                                                 |
| 63                    | 63 91%                            |                                                 |
| 64                    | 66 98%                            | 74 94%                                          |
| 65                    | 67 98%                            | 75 93%                                          |
| 68                    | 68 98%                            |                                                 |
| 69                    | 70 97%                            |                                                 |
| 70                    | 69 99%                            | 76 98%                                          |
| 71                    | 72 98%                            | 77 96%                                          |
| 72                    | 71 75%                            | 78 95%                                          |
| 73                    | 73 98%                            | 79 98%                                          |
| 74                    | 76 75%                            | 81 92%                                          |
| 75                    | 75 98%                            | 80 94%                                          |
| 76                    | 76 87%                            | 82 91%                                          |
| 77                    | 77 99%                            | 86 98%                                          |

|     |     |      |     |     |
|-----|-----|------|-----|-----|
| 78  | 79  | 98%  | 88  | 93% |
| 79  | 80  | 99%  | 89  | 96% |
| 80  | 78  | 96%  | 90  | 93% |
| 81  | 81  | 98%  | 93  | 95% |
| 82  | 82  | 97%  | 94  | 96% |
| 83  | 83  | 99%  | 95  | 97% |
| 84  | 84  | 100% | 96  | 99% |
| 85  | 85  | 99%  | 97  | 97% |
| 86  | 86  | 97%  |     |     |
| 87  | 87  | 98%  |     |     |
| 88  | 88  | 96%  | 99  | 81% |
| 89  | 89  | 96%  | 98  | 79% |
| 90  | 90  | 99%  | 100 | 97% |
| 91  | 91  | 100% | 101 | 89% |
| 92  | 92  | 99%  | 104 | 96% |
| 93  | 94  | 99%  | 105 | 98% |
| 94  | 93  | 94%  | 106 | 98% |
| 95  | 95  | 95%  | 107 | 97% |
| 96  | 96  | 99%  | 108 | 93% |
| 97  | 97  | 99%  | 109 | 94% |
| 98  | 98  | 90%  |     |     |
| 99  | 99  | 97%  |     |     |
| 100 | 101 | 89%  |     |     |
| 101 | 100 | 96%  |     |     |
| 102 | 102 | 92%  |     |     |
| 103 | 103 | 93%  |     |     |
| 104 | 104 | 90%  |     |     |
| 105 | 106 | 88%  |     |     |
| 106 | 105 | 81%  | 114 | 78% |
| 108 | 107 | 99%  | 115 | 98% |
| 109 | 109 | 87%  |     |     |
| 110 | 110 | 99%  | 116 | 97% |
| 111 | 113 | 99%  | 117 | 97% |
| 112 | 111 | 98%  | 119 | 96% |
| 113 | 112 | 96%  | 118 | 94% |
| 114 | 114 | 99%  | 120 | 93% |
| 115 | 115 | 99%  | 121 | 91% |
| 116 | 116 | 98%  | 122 | 92% |
| 117 | 117 | 98%  | 123 | 92% |
| 118 | 118 | 98%  | 124 | 97% |
| 119 | 119 | 98%  | 125 | 97% |

---

Table S14: Identification of symmetry pairs of vibrational modes between 500–2000  $\text{cm}^{-1}$  in the three derivatives. Mode displacement vector overlap between A-type and symmetrized B-type modes are given in percent. Only modes with dominant overlaps over 80% are shown.

| Pt(Me-BPCH) |      | Au(Me-BPCH) |      | Pt(CF <sub>3</sub> -BPCH) |      |
|-------------|------|-------------|------|---------------------------|------|
| 35/36       | 90%  | 34/35       | 81%  | 42/43                     | 90%  |
| 38/39       | 92%  | 38/39       | 82%  | 50/51                     | 91%  |
| 42/43       | 84%  | 42/43       | 85%  | 54/55                     | 97%  |
| 44/45       | 90%  | 44/45       | 95%  | 56/57                     | 94%  |
| 46/47       | 95%  | 46/47       | 96%  | 62/63                     | 96%  |
| 49/50       | 94%  | 51/52       | 97%  | 68/69                     | 100% |
| 58/59       | 100% | 58/59       | 100% | 72/73                     | 98%  |
| 62/63       | 87%  | 62/63       | 96%  | 74/75                     | 100% |
| 64/65       | 100% | 64/65       | 96%  | 80/81                     | 92%  |
| 66/67       | 97%  | 66/67       | 100% | 83/84                     | 97%  |
| 68/69       | 100% | 68/70       | 100% | 85/87                     | 87%  |
| 75/76       | 84%  | 75/76       | 99%  | 88/89                     | 95%  |
| 78/79       | 100% | 79/80       | 100% | 98/99                     | 96%  |
| 86/87       | 95%  | 86/87       | 97%  | 103/104                   | 86%  |
| 88/89       | 92%  | 88/89       | 95%  | 112/113                   | 100% |
| 91/92       | 87%  | 91/92       | 85%  | 114/115                   | 80%  |
| 100/101     | 81%  | 100/101     | 91%  | 118/119                   | 100% |
| 102/103     | 96%  | 102/103     | 97%  | 120/121                   | 100% |
| 104/105     | 89%  | 104/106     | 89%  | 122/123                   | 100% |
| 112/113     | 97%  | 111/112     | 89%  | 124/125                   | 99%  |
| 114/115     | 100% | 114/115     | 100% |                           |      |
| 116/117     | 100% | 116/117     | 100% |                           |      |
|             |      | 118/119     | 99%  |                           |      |

## PV potential curve comparisons

Table S15: Comparison of the potential energy curves  $V$  (blue lines) and the PV potential curves  $V^{PV}$  for selected related vibrational modes of Pt(Me-BPCH), Au(Me-BPCH) and Pt(CF<sub>3</sub>-BPCH). The modes are grouped into symmetry related pairs where possible and are aligned such that the displacement vectors (i.e. the  $q$  axes) are oriented in the same direction.

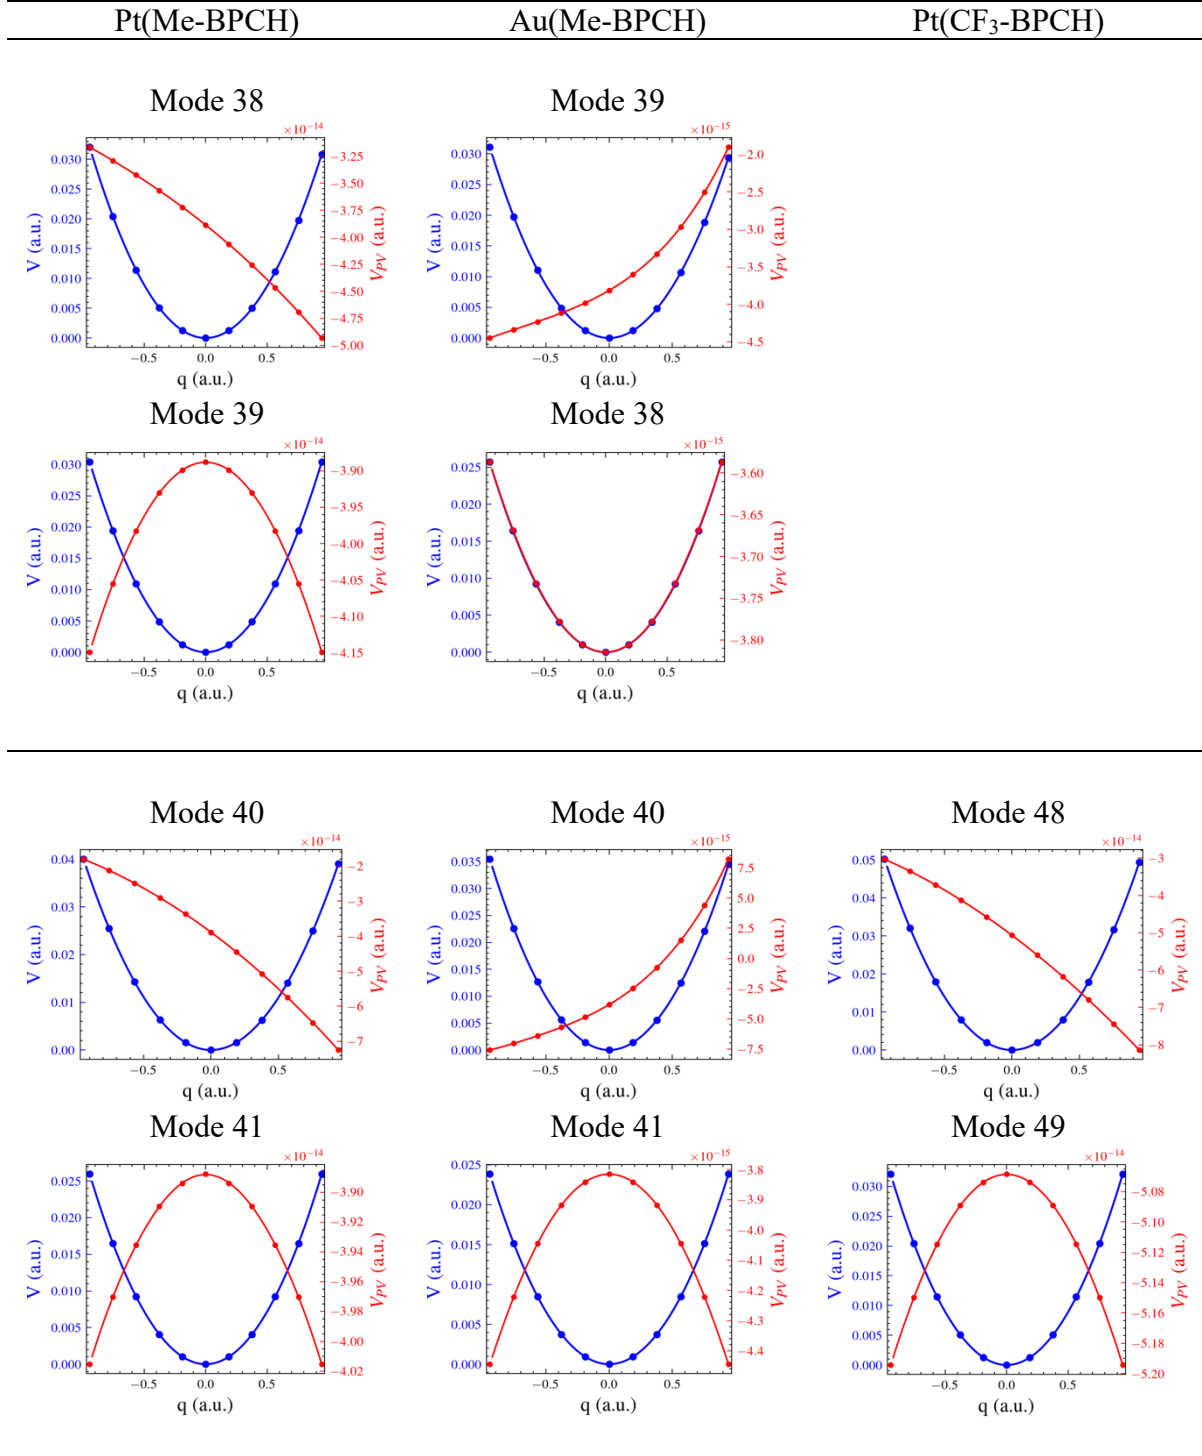

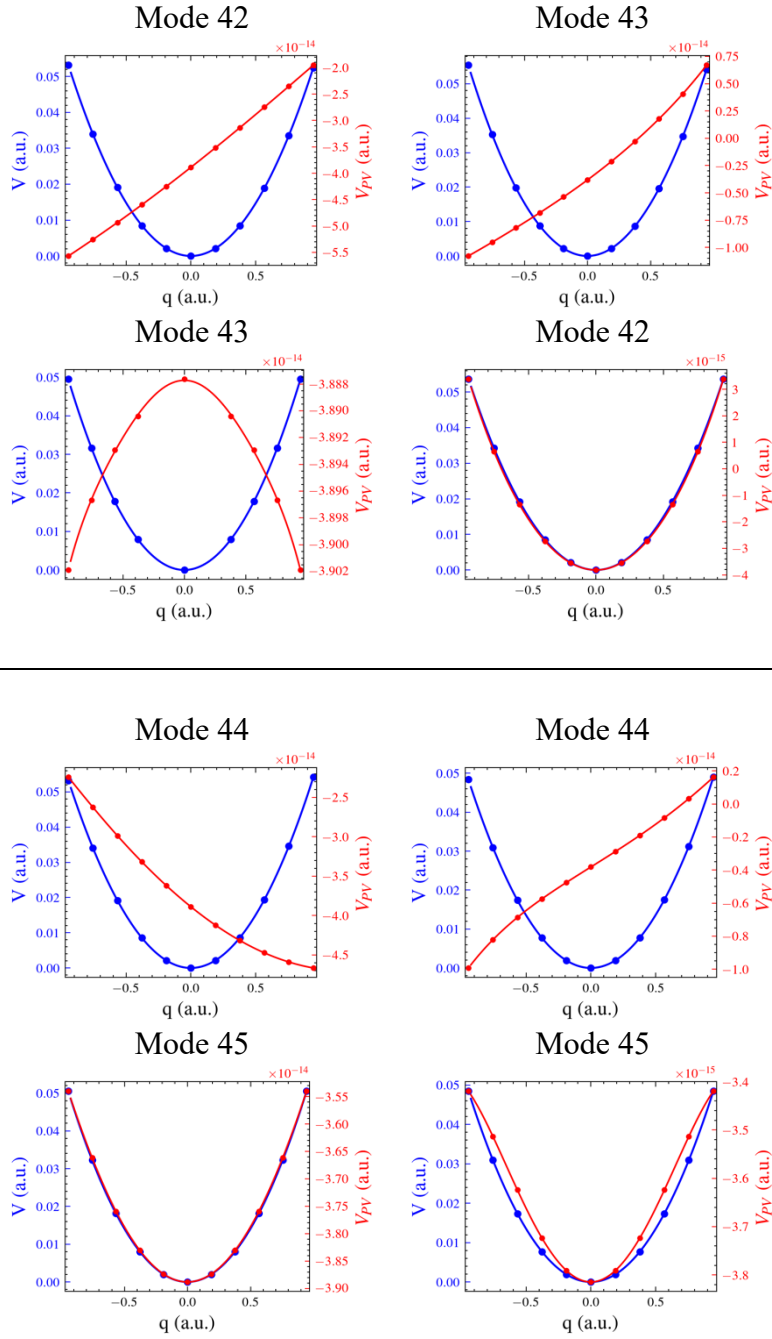

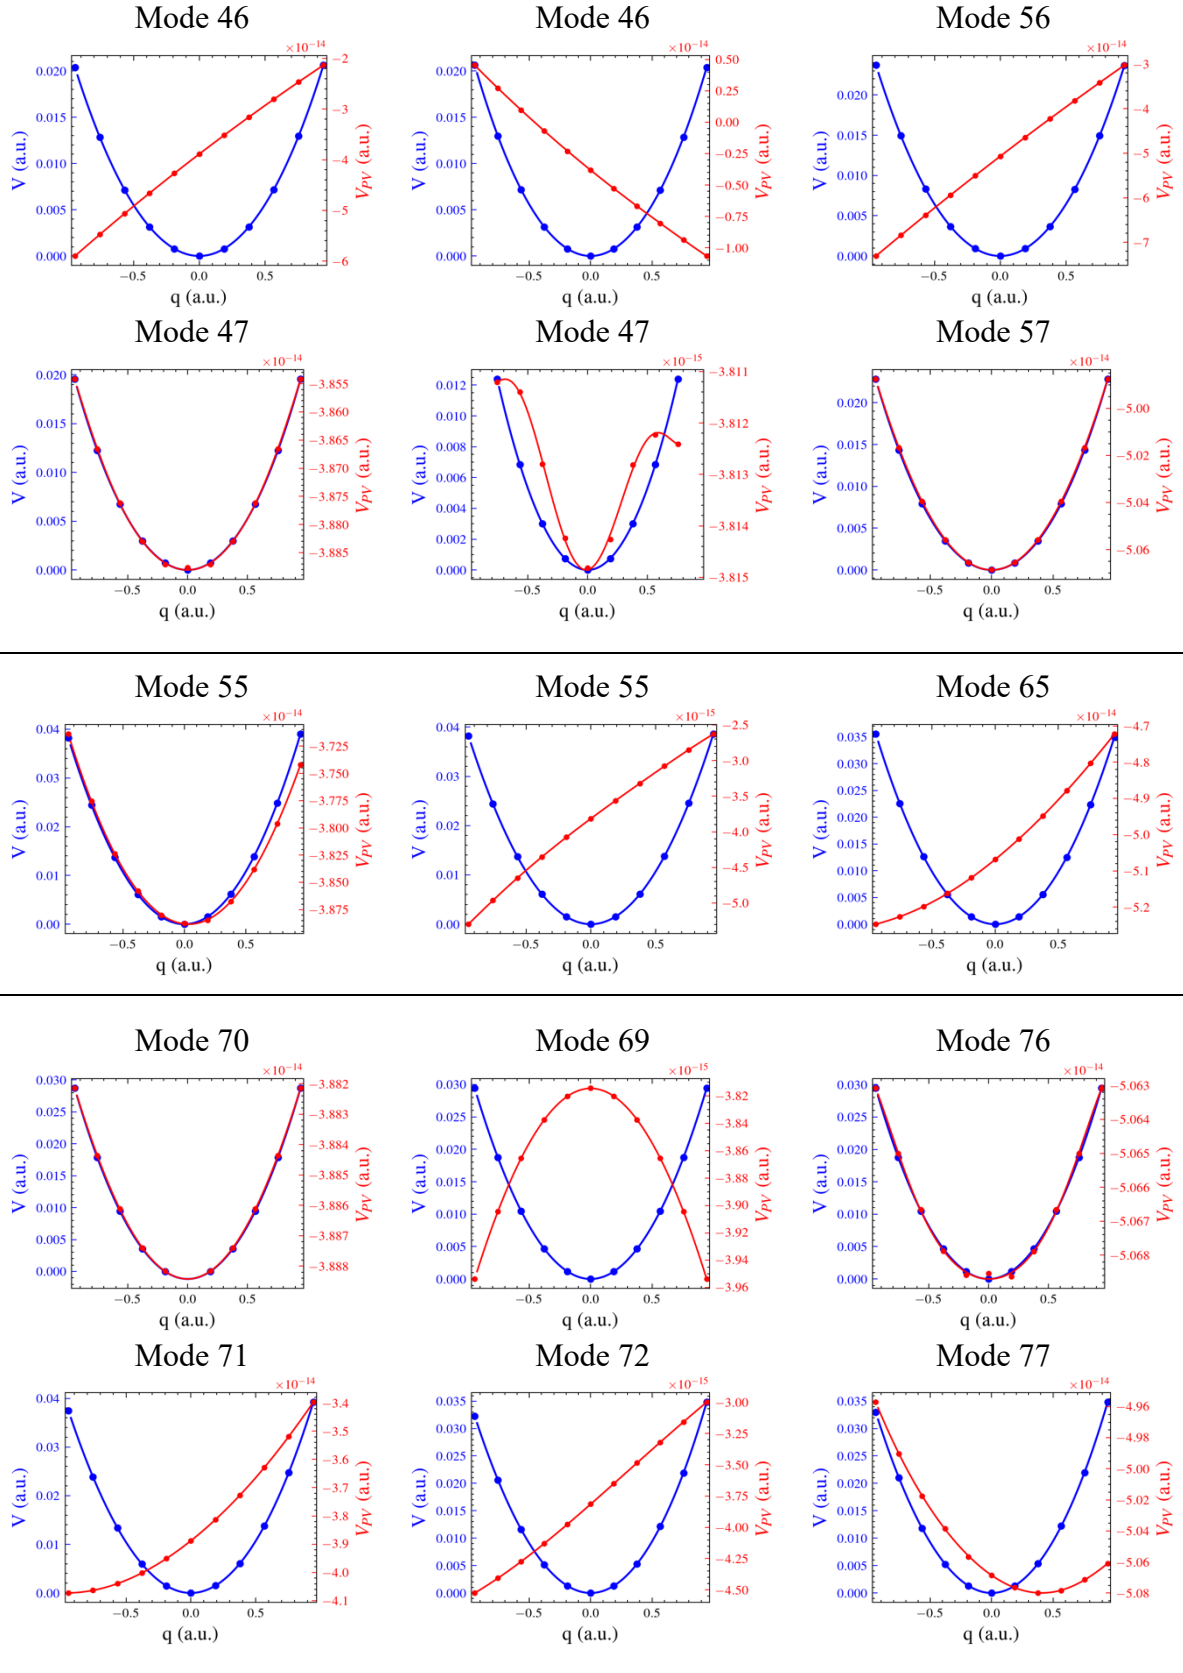

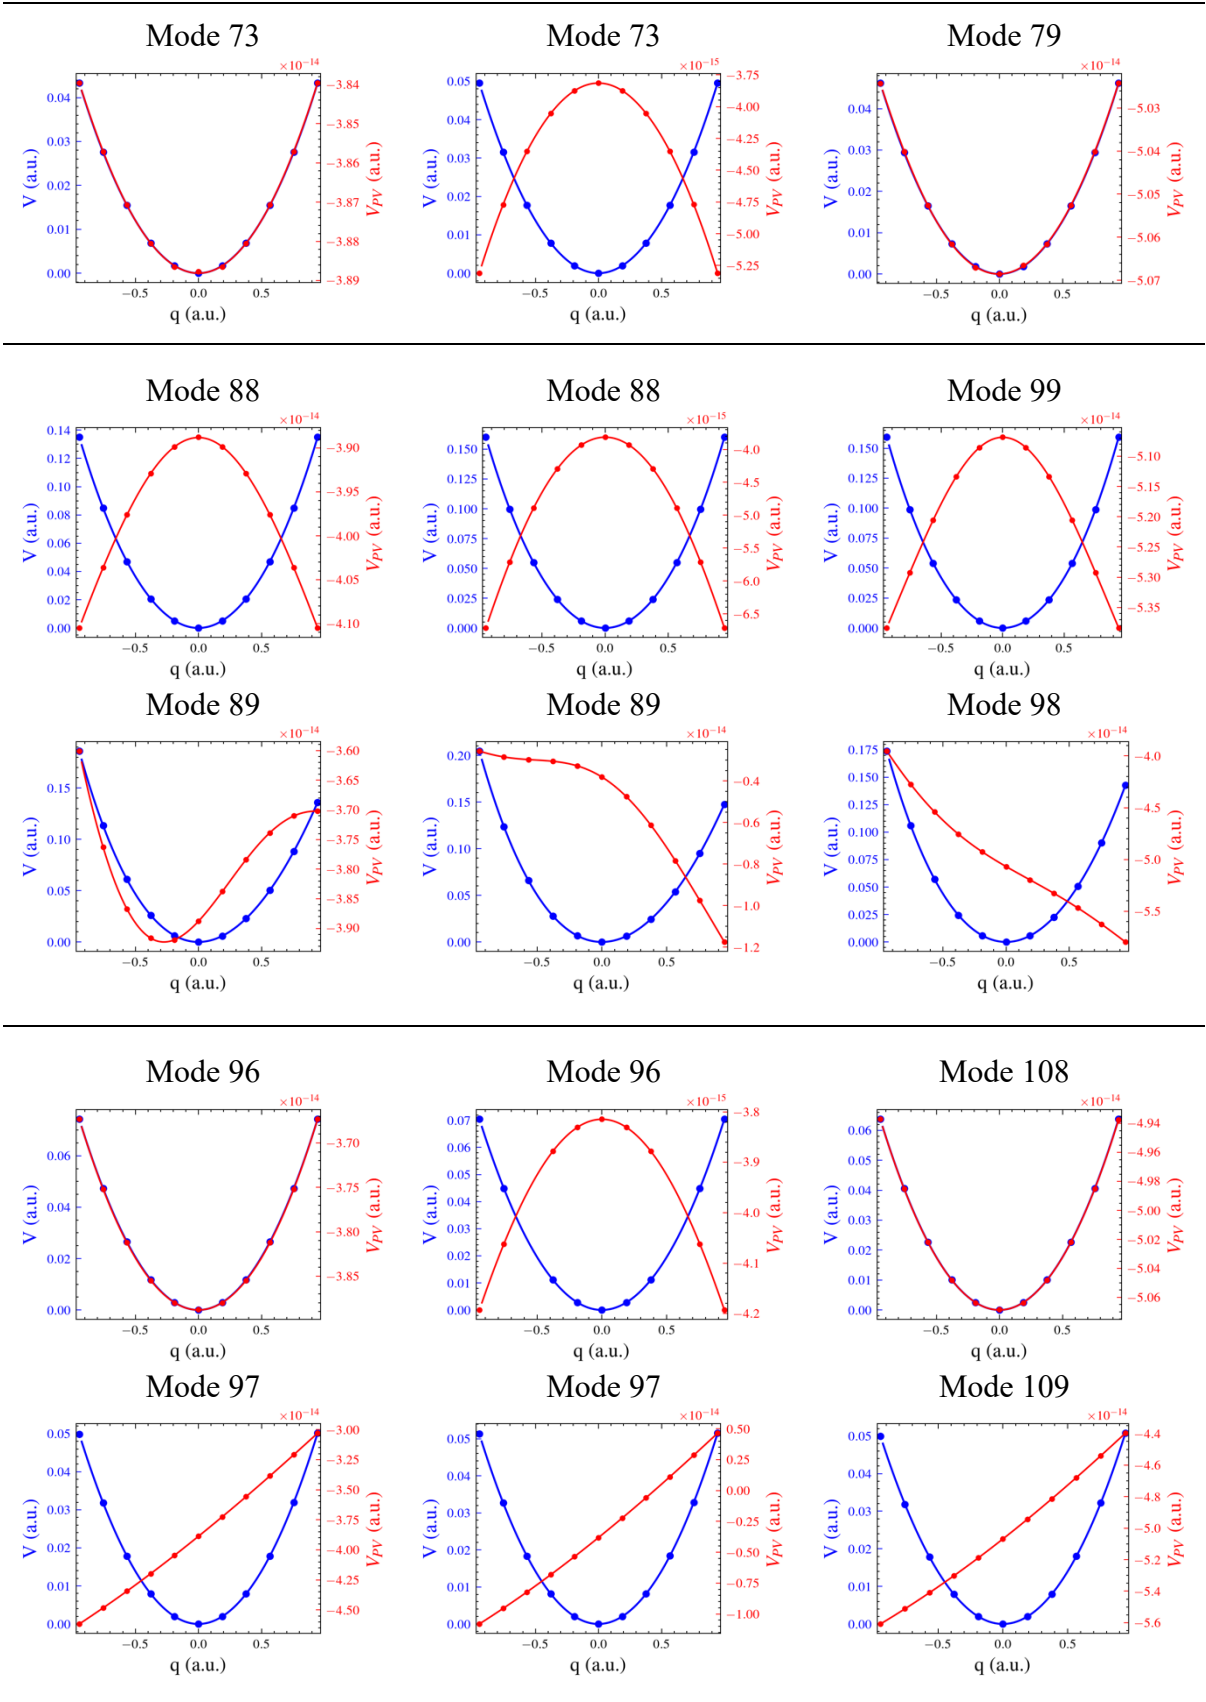

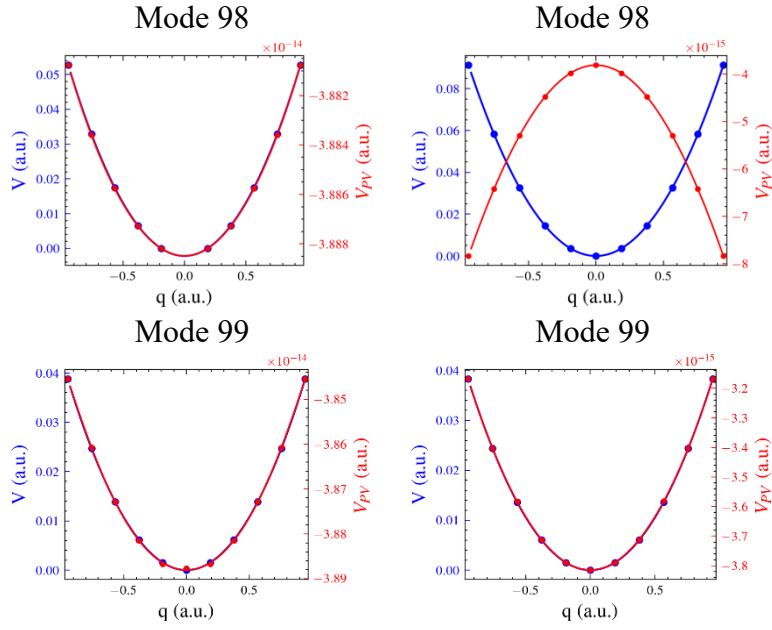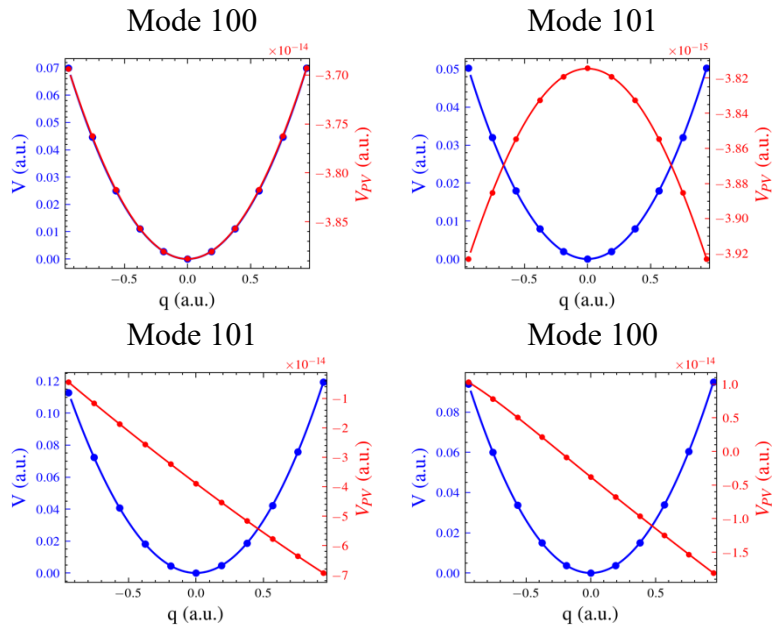



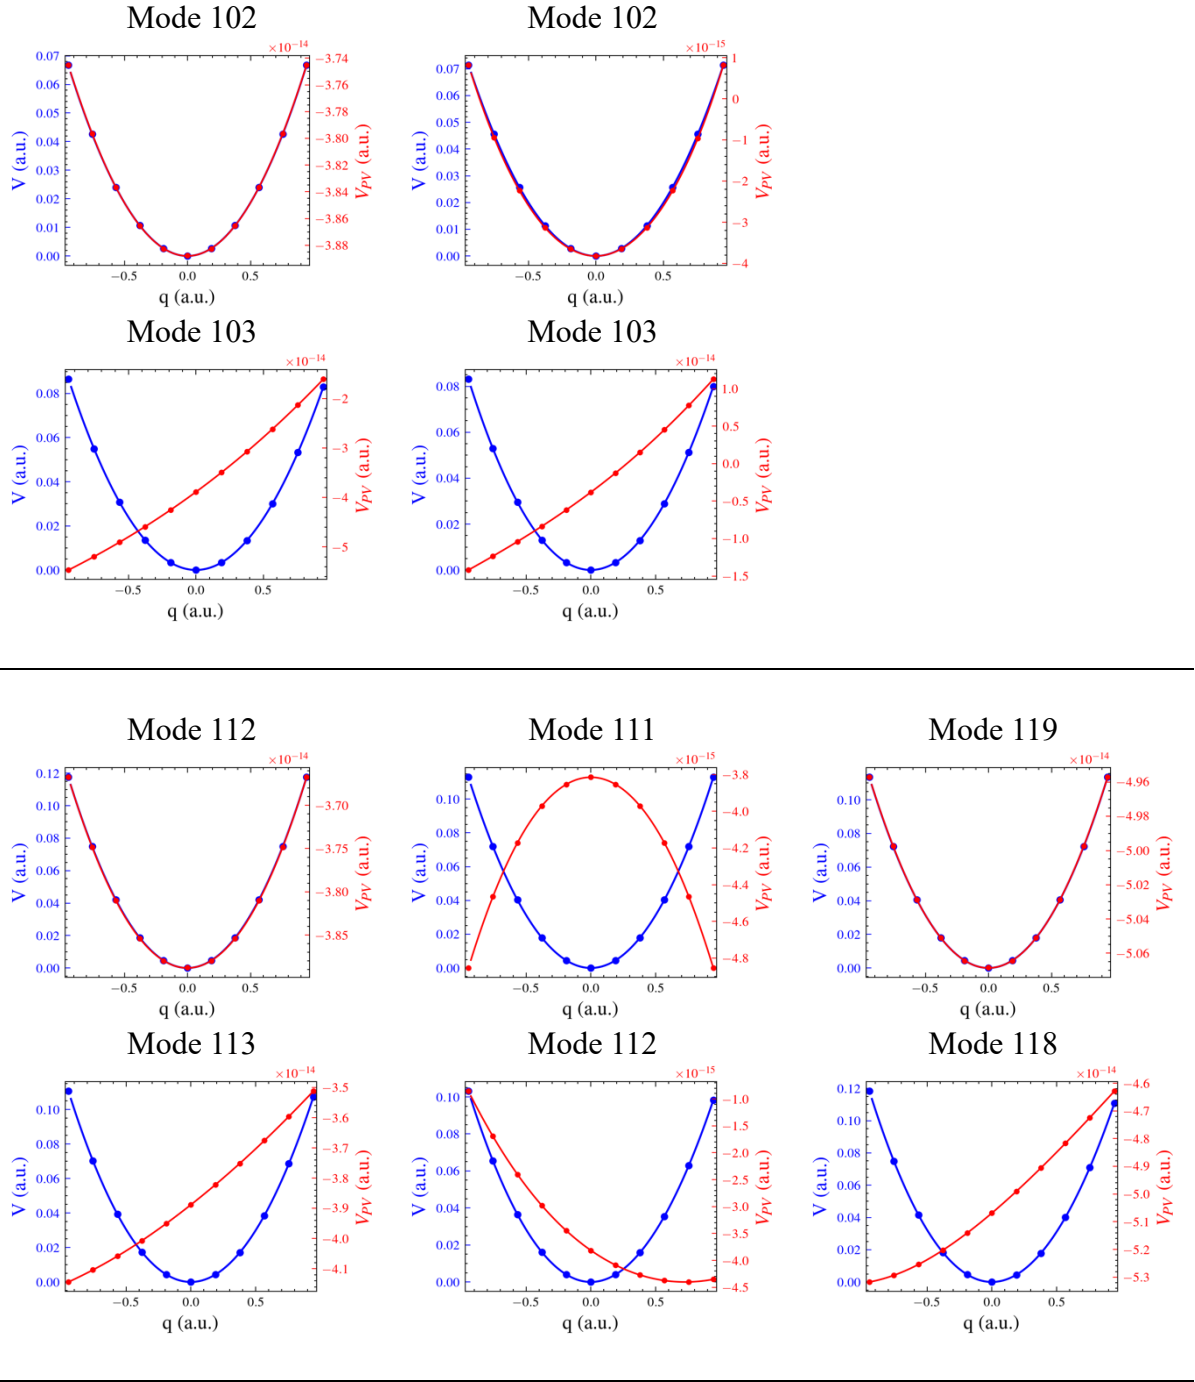

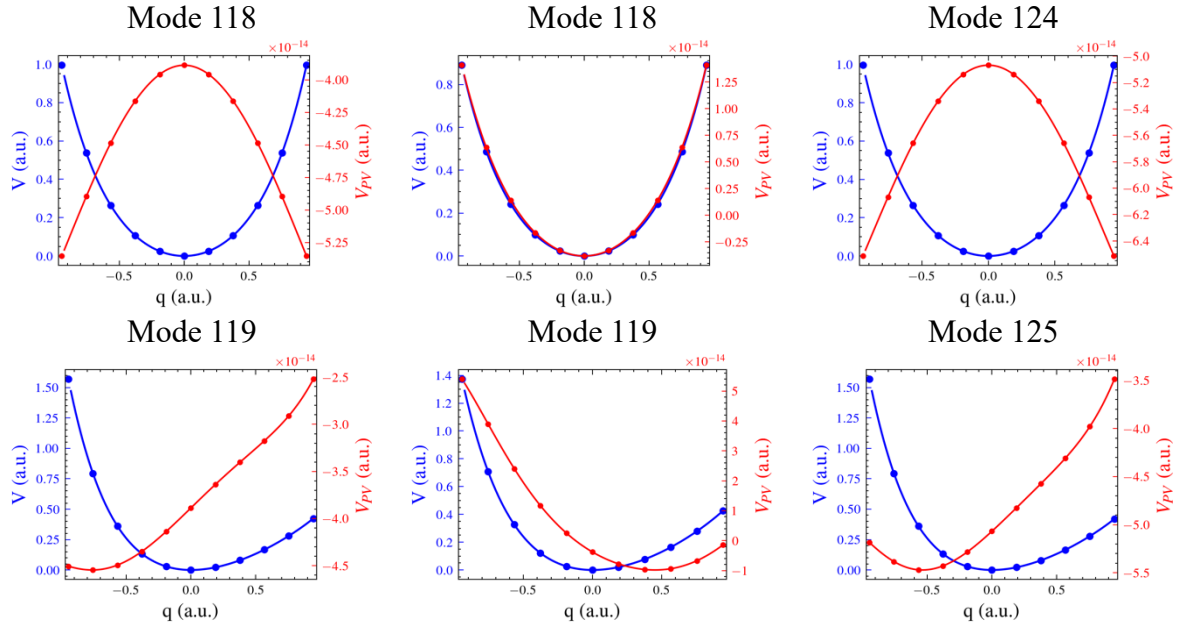

## References

- [1] Bateman, L.; Breeden, S. W.; O'Leary, P. New chiral diamide ligands synthesis and applications in allylic alkylation. *Tetrahedron: Asymmetry*. **2008**, 19, 391-396. DOI: 10.1016/j.tetasy.2008.01.018
